# Supplementary material for: Classical and quantum reservoir computing: development and applications in machine learning
Source: arXiv:2310.07455 source file (2023-10-11)
Supplement: Supplementary file 1 [file appendix4.tex]

%%%%%%%%%%%%%%%%%%%%%%%%%%%%%%%%%%%%%%%%%%%%%%%%%%%%%%%%%
% CONFIDENCE INTERVAL PREDICTION
%%%%%%%%%%%%%%%%%%%%%%%%%%%%%%%%%%%%%%%%%%%%%%%%%%%%%%%%%

\section{Confidence intervals prediction}
\label{sect:intervals}
\CR{REVISAD EL RESTO DEL CAPÍTULO MÁS A FONDO, POR FAVOR, YA QUE ESTA PARTE NO SE HA REVISADO ANTES (NO LO HEMOS MANDADO AÚN A PUBLICAR)}\\
\\
Quantifying the uncertainties associated with deterministic forecasting of financial time series is essential to enhance the reliability of many business decisions, as it provides deeper insight into the performance of ML models.

Interval prediction \cite{interval_prediction} is a method that quantifies the uncertainty of forecasts by presenting the predicted lower and upper limits at a particular prediction interval nominal confidence (\gls{PINC}) level. High-quality prediction intervals are defined as the those that cover a specified proportion of the observations while still being as narrow as possible. Indeed, under the same level of PINC, narrower prediction intervals can provide more accurate information with fewer uncertainties. 

In this study, we present a method based on modeling the distribution of forecasting errors made by the D-RC algorithm, whose results were presented before, during training phase. As we have seen in the previous sections, the agricultural financial time series are particularly volatile, and thus present abrupt changes of tendency. As a consequence, we expect the error distribution to exhibit different behavior depending on whether or not there is a significant change of tendency in the predictions. For this reason, the training data has been separated in three sets according to the relative increase of the prices. That is, let $y_\text{teach}(t)$ be the actual time series at time $t$ and $y(t)$ be the prediction by the D-RC model. Then, the first set contains the data with relative increase is higher than +10\% (Increase). The second class contains the data with relative increase lower than -10\% (Decrease). Finally the third set contains the data with relative increase between -10\% and +10\% (Constant):
\begin{eqnarray}
   &\text{Increase} \rightarrow &\displaystyle \frac{y_\text{teach}(t-1) - y(t)}{y(t)} \geq 0.1, \\ \nonumber
   &\text{Decrease} \rightarrow &\displaystyle \frac{y_\text{teach}(t-1) - y(t)}{y(t)} \leq -0.1, \\ \nonumber
   &\text{Constant} \rightarrow & -0.1 < \displaystyle \frac{y_\text{teach}(t-1) - y(t)}{y(t)} < 0.1.
   \label{eq:interval_definition}
\end{eqnarray}
Once the training data has been divided into these three sets, the error distribution $\epsilon(t) = y(t) - y_\text{teach}(t)$ is studied. Then, we find the best fit for the probability distribution. In this case, all distributions are modeled using a Normal Inverse Gaussian (\gls{NIG}) distribution \cite{norminvgaus}, whose probability density function is given by:
\begin{equation}
    f(x,a,b) = \frac{a K_1(a\sqrt{1+y^2})}{\pi \sqrt{1 + y^2}}e^{\sqrt{a^2 - b^2} + by}, \quad y= \frac{x - x_0}{\sigma},
\end{equation}
where $x$ is a real number, the parameter $a$ is the tail heaviness and $b$ is the asymmetry parameter satisfying $a>0$ and $|b| \leq a$, $x_0$ and $\sigma$ are the location and scale factors and $K_1$ is the modified Bessel function of second kind \cite{bessel}. Then, the resulting probability distribution is used to calculate the lower and upper bounds of the prediction interval at a given probability level PINC:
\begin{eqnarray}
    U_t = y(t) + \text{NIG}_k(\text{PINC}/2), \quad L_t = y(t) + \text{NIG}_k(1-\text{PIC}/2), \\ \nonumber
    \quad k \in \{\text{\emph{Constant}, \emph{Increase}, \emph{Decrease}}\}.
\end{eqnarray}
After calculating the confidence intervals $[L_t, U_t]$ for the validation/testing steps $t=1, \cdots, T$, two metrics are used to evaluate the quality of such intervals. The first one is the Average Coverage Error (\gls{ACE}), which measures how much the predicted intervals can be trusted. 
\begin{equation}
    \text{ACE} = \text{PICP} - \text{PINC}, \quad \text{PICP}=\frac{1}{T} \sum_{t=1}^T c_t, \quad c_t = \left\{\begin{array}{ll} 
    1 & \text{if } y_\text{teach}(t) \in [L_t, U_t]\\
    0 & \text{otherwise},
    \end{array} 
\right.
\end{equation}
where \gls{PICP} is the Prediction Interval Coverage Probability. The second metric is the Prediction Interval Average Width (\gls{PIAW}), which measures the average width of the predicted intervals:
\begin{equation}
    \text{PIAW} = \frac{1}{T} \sum_{t=1}^T (U_t - L_t).
\end{equation}
The predicted intervals should be as narrow as possible, meaning they should minimize the PIAW, while following the condition $\text{ACE} \geq 0$. In the following sections we present and evaluate the predicted intervals for the three time series at study: zucchini, aubergine and tomato.

\begin{table}[!t]
    \centering
    \begin{tabular}{c|cccc}
    \hline\hline \\[-0.3cm]
          Time series & Set & Distribution & Squared Error &  BIC \\
          \hline \\[-0.2cm]
         \multirow{6}{*}{Zucchini} & \multirow{2}{*}{Constant} & NIG & 94 &  276 \\
         & &  Gaussian & 109 &  286 \\[0.3cm]
          & \multirow{2}{*}{Increase} & NIG & 88  & -8.3 \\
         & &  Gaussian & 98 &  -7.0 \\[0.3cm]
         & \multirow{2}{*}{Decrease} & NIG & 74 & -44 \\
         & &  Gaussian & 78 & -42 \\[0.3cm]
         \hline \\[-0.2cm]
         \multirow{6}{*}{Aubergine} & \multirow{2}{*}{Constant} & NIG & 80  & -23 \\
         & &  Gaussian & 134 &  18 \\[0.3cm]
          & \multirow{2}{*}{Increase} & NIG & 74  & -40 \\
         & &  Gaussian & 80 & -40 \\[0.3cm]
         & \multirow{2}{*}{Decrease} & NIG & 134  & 23 \\
         & &  Gaussian & 159 & 35 \\[0.3cm]
         \hline \\[-0.2cm]
         \multirow{6}{*}{Tomato} & \multirow{2}{*}{Constant} & NIG & 98 &  -18 \\
         & &  Gaussian & 122 &  1.7 \\[0.3cm]
          & \multirow{2}{*}{Increase} & NIG & 55  & -65 \\
         & &  Gaussian & 83 &  -28 \\[0.3cm]
         & \multirow{2}{*}{Decrease} & NIG & 141 & 37 \\
         & &  Gaussian & 155  & 39 \\[0.3cm]
         \hline 
    \end{tabular}
    \caption{Squared error and BIC indicators for the Normal Inverse Gaussian (NIG) distribution for the three time series and relative increase sets, compared with the Gaussian distribution.}
    \label{tab:best_distribution_params}
\end{table}

\subsection*{Zucchini}
\begin{figure}[!ht]
\centering
\includegraphics[width=1.0\textwidth]{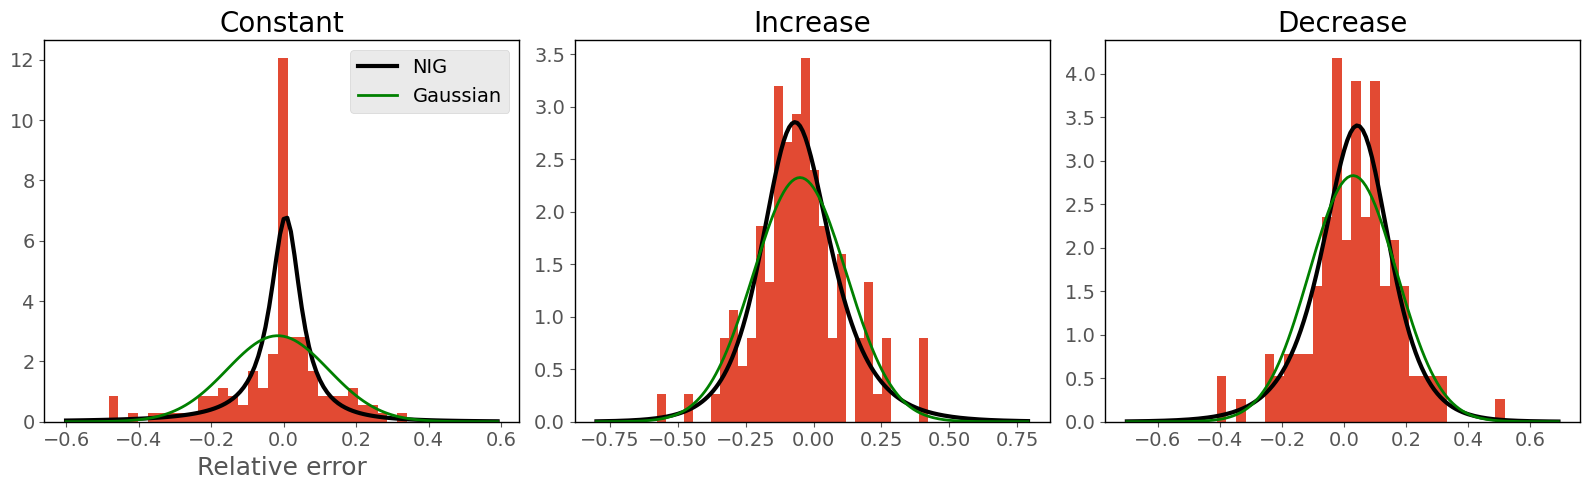}
\caption{Distribution of the relative error in the training set for the \emph{Constant} set (left), the \emph{Increase} set (center) and the \emph{Decrease} set (right). See Eq. \ref{eq:interval_definition} for the definition of the three sets. }
\label{fig:dist_zucchini}
\end{figure}

The relative error distributions for the training set are shown in Fig. \ref{fig:dist_zucchini}. As can be seen, the relative error is significantly smaller for the set containing the \emph{Constant} distribution (see Eq. \ref{eq:interval_definition}). Moreover, the \emph{Increase} distribution has positive skewness, while the \emph{Decrease} distribution has negative skewness. This skewness agrees with the definition of the three sets and means that the predictions tend to underestimate big changes of tendency in the data. The distributions in Fig. \ref{fig:dist_zucchini} are modeled using a NIG with parameters $a=0.12$, $b=-0.048$, $x_0=0.0069$, $\sigma=0.051$ for the \emph{Constant} set, $a=1.36$, $b=0.22$, $x_0=-0.083$, $\sigma=0.20$ for the \emph{Increasing} set and $a=1.66$, $b=-0.25$, $x_0=0.056$, $\sigma=0.18$ for the \emph{Decreasing} set. The NIG distribution is chosen among other distributions since it minimizes the BIC (Bayesian Information Criterion) indicator and the squared error, which are given in Table \ref{tab:best_distribution_params}. The BIC indicator measures the quality of a statistical model while taking into account the balance between goodness of fit and model complexity \cite{AIC_BIC}. Figure \ref{fig:dist_zucchini} shows the shape of the fitted distribution together with the best fit of the Gaussian distribution. As can be seen, the difference of both distributions is specially relevant for the \emph{Constant} set, where the Gaussian distribution does not capture the peak around $\epsilon=0$. 
\begin{figure}[!ht]
\centering
\includegraphics[width=1.0\textwidth]{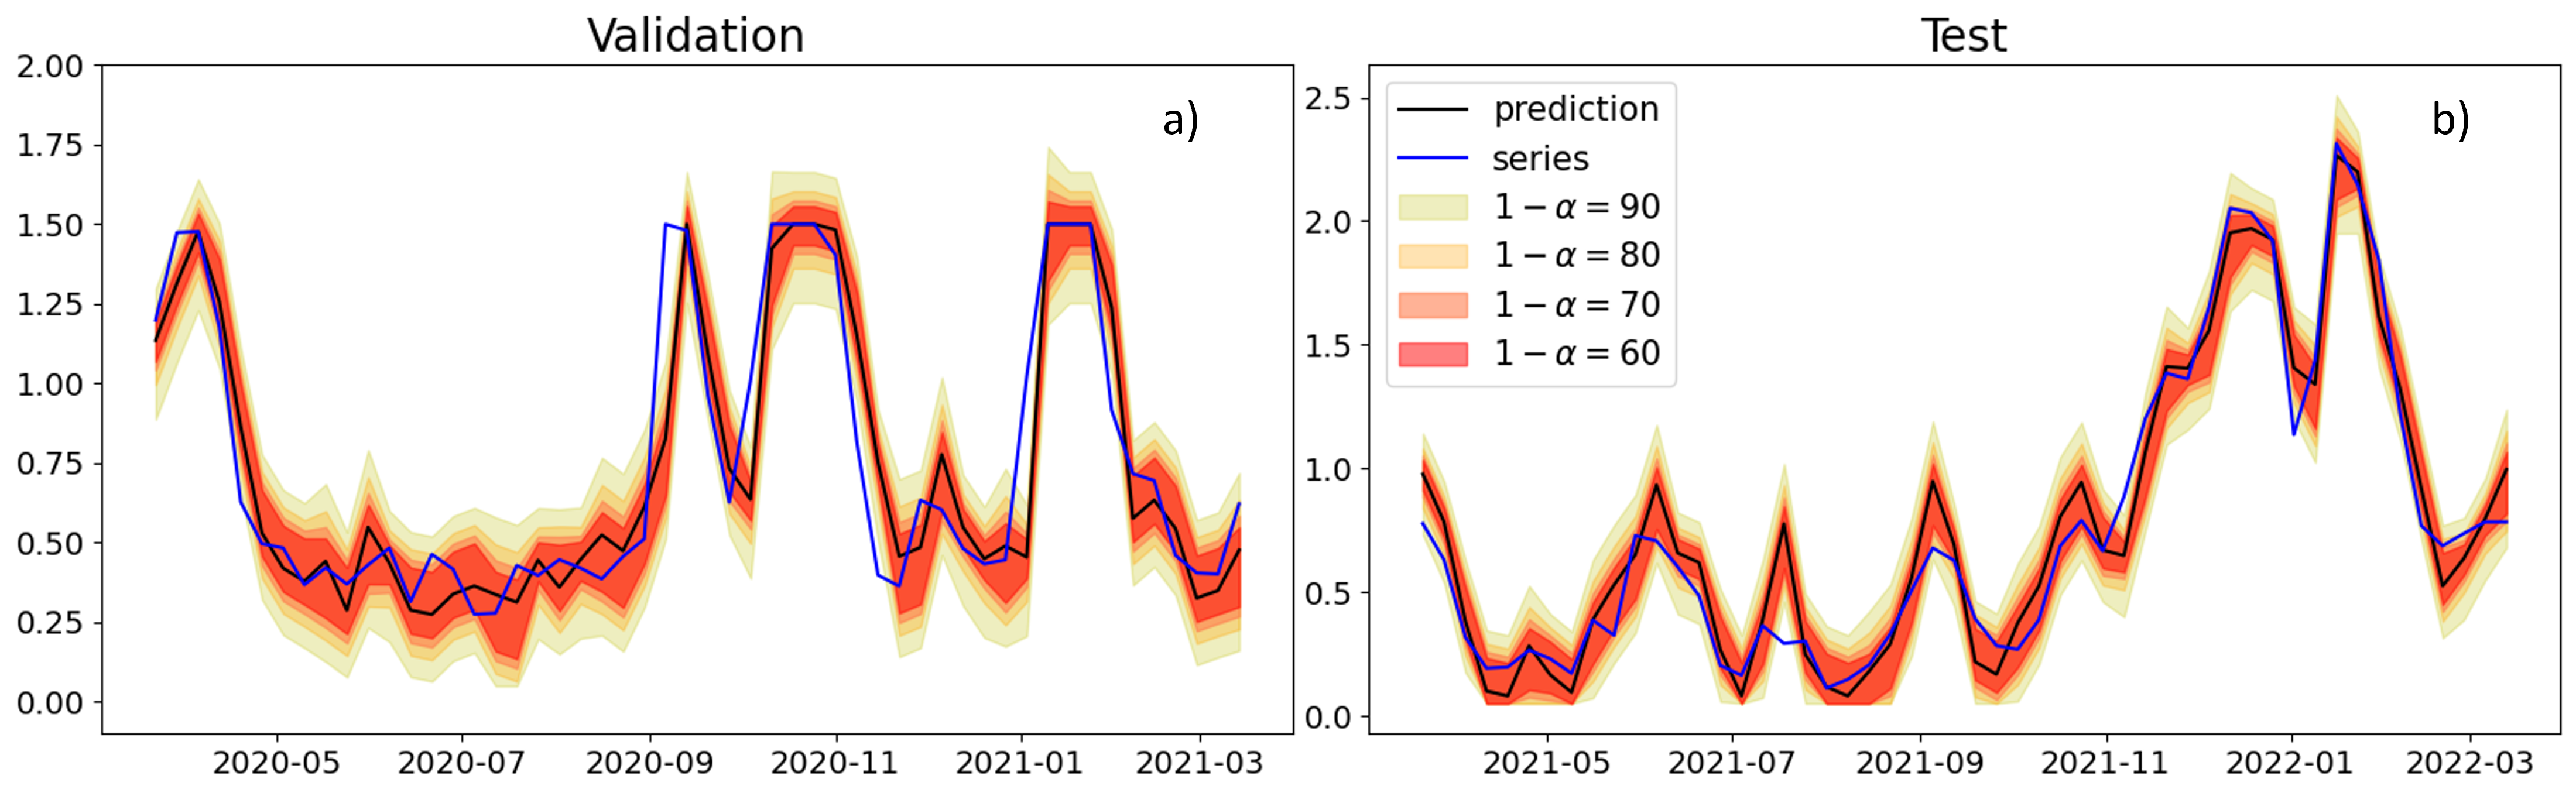}
\caption{Predicted confidence interval for the zucchini time series for the validation and test set.}
\label{fig:intervals_zucchini}
\end{figure}
The fitted distributions have been used to construct the predicted confidence intervals for four different values of PINC=90\%, 80\%, 70\% and 60\%. The intervals for the validation and test set are displayed in Fig. \ref{fig:intervals_zucchini}, where it can be observed that most of the target values are enclosed by these constructed prediction intervals. The PICP, ACE and PIAW for both the NIG and Gaussian distributions are given in Table \ref{tab:intervals_zucchini}. As can be seen, the condition of $ACE \gtrapprox  0$ is almost always accomplished, except for PINC=60\%, where the ACE for the NIG distribution is slighlty smaller than 0. The Gaussian distribution tends to have higher values of ACE but also higher values of PIAW, which means that such distribution is overestimating the size of the confidence intervals. Thus, the predicted Gaussian intervals are less informative than the predicted NIG intervals, verifying the superiority of the NIG distribution over the Gaussian distribution.

\begin{table}[!ht]
    \centering
    \begin{tabular}{cccccccc}
    \hline \hline\\[-0.3cm]
                      &  \multicolumn{6}{c}{ \textbf{Z U C C H I N I}} &\\
                        \cmidrule(lr){2-4}\cmidrule(lr){5-7}
                       \cmidrule(lr){2-7}
                      & & \multicolumn{3}{c}{Validation} &  \multicolumn{3}{c}{Test}\\
                        \cmidrule(lr){3-5}\cmidrule(lr){6-8}
        %\hline
         PINC  & Distribution   & PICP & ACE & PIAW & PICP & ACE & PIAW\\
        \hline \\[-0.3cm]
        \multirow{ 2}{*}{90\%} & NIG & 0.865 & -0.035   & 0.469 & 0.942 & 0.042 & 0.458 \\
        & Gaussian & 0.895 & -0.005 & 0.489 & 0.942& 0.042 & 0.475 \\
        \hline \\[-0.3cm]
        \multirow{ 2}{*}{80\%} & NIG   & 0.846 & 0.046 & 0.324   & 0.846 & 0.046 & 0.328 \\
        & Gaussian &  0.865 & 0.065 & 0.383 & 0.904 & 0.104 & 0.376\\
        \hline \\[-0.3cm]
        \multirow{ 2}{*}{70\%} & NIG  & 0.731 & 0.031 & 0.246   & 0.712   & 0.012 & 0.254 \\
        & Gaussian & 0.769 & 0.069& 0.310 & 0.846 & 0.146 & 0.308\\
        \hline \\[-0.3cm]
        \multirow{ 2}{*}{60\%} & NIG & 0.577 & -0.023 & 0.191   & 0.577   & -0.023 & 0.201 \\
        & Gaussian & 0.731 & 0.131 & 0.251 & 0.635 & 0.035 & 0.252\\
         \hline
    \end{tabular}
    \caption{Prediction Interval Nominal Coverage (PINC), Prediction Interval Coverage Probability (PICP), Average Coverage Error (ACE) and Prediction Interval Average Width (PIAW) for the interval prediction for the validation and test sets for the zucchini time series, compared with the Gaussian distribution.}
    \label{tab:intervals_zucchini}
\end{table}

\subsection*{Aubergine}
\begin{figure}[!ht]
\centering
\includegraphics[width=1.0\textwidth]{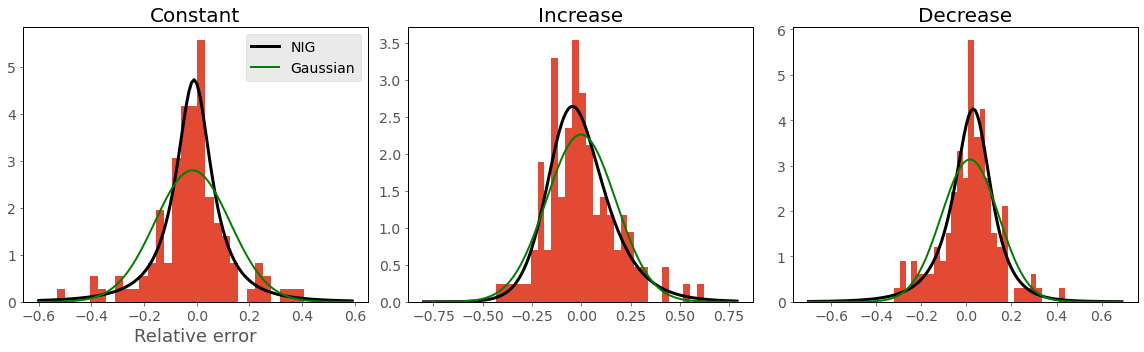}
\caption{Same as Fig. \ref{fig:dist_zucchini} for the aubergine series. }
\label{fig:dist_aubergine}
\end{figure}

The previous analysis is repeated for the aubergine time series. The relative error distributions are shown in Fig. \ref{fig:dist_aubergine}. In this case, the distributions are modeled using a NIG with parameters $a=0.31$, $b=-0.025$, $x_0=-0.0097$, $\sigma=0.084$ for the \emph{Constant} set, $a=2.68$, $b=1.05$, $x_0=-0.11$, $\sigma=0.257$ for the \emph{Increasing} set and $a=0.77$, $b=-0.14$, $x_0=0.037$, $\sigma=0.11$ for the \emph{Decreasing} set. The BIC and squared error for this distributions, compared with the normal distributions, are given in Table \ref{tab:best_distribution_params}. In this case, the distribution for the \emph{Constant} set also has smaller variance. The \emph{Increase} distribution has positive skewness and the \emph{Decrease} distribution has negative skewness, which is captured by the NIG distribution but not by the Gaussian distribution. The resulting predicted intervals are shown in Fig. \ref{fig:intervals_aubergine}. Again, most of the predictions lie within the confidence intervals. The metrics to evaluate such intervals are given in Table \ref{tab:intervals_aubergine}. The results are qualitatively equivalent to those from the zucchini time series. That is, the predicted Gaussian intervals are less informative than the predicted NIG intervals because  the Gaussian distribution produces too wide confidence intervals, while the NIG distribution is more suitable for estimating the relative error.

\begin{figure}[!ht]
\centering
\includegraphics[width=1.0\textwidth]{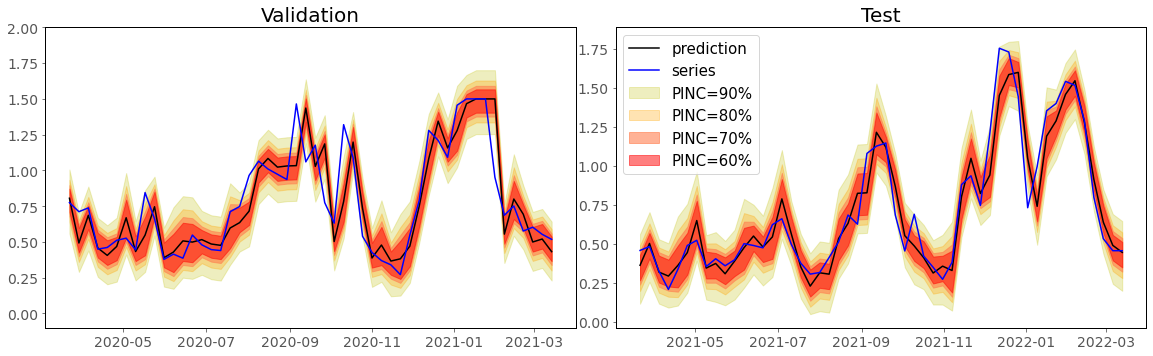}
\caption{Predicted confidence interval for the aubergine time series for the validation and test set.}
\label{fig:intervals_aubergine}
\end{figure}

\begin{table}[!ht]
    \centering
    \begin{tabular}{cccccccc}
    \hline \hline\\[-0.3cm]
                      &  \multicolumn{6}{c}{ \textbf{A U B E R G I N E}} &\\
                        \cmidrule(lr){2-4}\cmidrule(lr){5-7}
                       \cmidrule(lr){2-7}
                      & & \multicolumn{3}{c}{Validation} &  \multicolumn{3}{c}{Test}\\
                        \cmidrule(lr){3-5}\cmidrule(lr){6-8}
        %\hline
         PINC  & Distribution   & PICP & ACE & PIAW & PICP & ACE & PIAW\\
        \hline \\[-0.3cm]
        \multirow{ 2}{*}{90\%} & NIG & 0.865 & -0.035   & 0.470 & 0.942 & 0.042 & 0.475 \\
        & Gaussian & 0.846 & -0.054 & 0.485 & 0.942& 0.042 & 0.488 \\
        \hline \\[-0.3cm]
        \multirow{ 2}{*}{80\%} & NIG   & 0.807 & 0.007 & 0.327   & 0.866 & 0.065 & 0.335 \\
        & Gaussian &  0.826 & 0.027 & 0.378 & 0.9865 & 0.065 & 0.380\\
        \hline \\[-0.3cm]
        \multirow{ 2}{*}{70\%} & NIG  & 0.692 & -0.008 & 0.249   & 0.692   & -0.008 & 0.256 \\
        & Gaussian & 0.788 & 0.088& 0.305 & 0.846 & 0.146 & 0.308\\
        \hline \\[-0.3cm]
        \multirow{ 2}{*}{60\%} & NIG & 0.615 & 0.015 & 0.194   & 0.596   & -0.004 & 0.200 \\
        & Gaussian & 0.711 & 0.111 & 0.248 & 0.692 & 0.0092 & 0.202\\
         \hline
    \end{tabular}
    \caption{Same as Table \ref{tab:intervals_zucchini} for the aubergine time series.}
    \label{tab:intervals_aubergine}
\end{table}

\subsection*{Tomato}
Finally, the analysis is repeated for the tomato time series. The relative error distributions are shown in Fig. \ref{fig:dist_tomato}. In this case, the distributions are modeled using a NIG with parameters $a=0.699$, $b=0.074$, $x_0=0.0013$, $\sigma=0.094$ for the \emph{Constant} set, $a=0.508$, $b=0.192$, $x_0=-0.077$, $\sigma=0.093$ for the \emph{Increasing} set and $a=1.174$, $b=0.229$, $x_0=0.0022$, $\sigma=0.11$ for the \emph{Decreasing} set. The BIC and squared errors for this distributions, compared with the normal distributions, are given in Table \ref{tab:best_distribution_params}.  In this case, the distribution for the \emph{Constant} set also has smaller variance but this effect is less pronounced when compared with the other two time series. The predicted intervals resulting from this analysis are shown in Fig. \ref{fig:intervals_tomato}. Most of the predictions lie within the confidence intervals. The metrics to evaluate such intervals are given in Table \ref{tab:intervals_tomato}. Again, the results are qualitatively equivalent to those from the zucchini and aubergine time series, confirming the hypothesis of the NIG distribution being more suitable than the Gaussian distribution in modeling the error of the D-RC model.

\begin{figure}[!ht]
    \centering
    \includegraphics[width=1.0\textwidth]{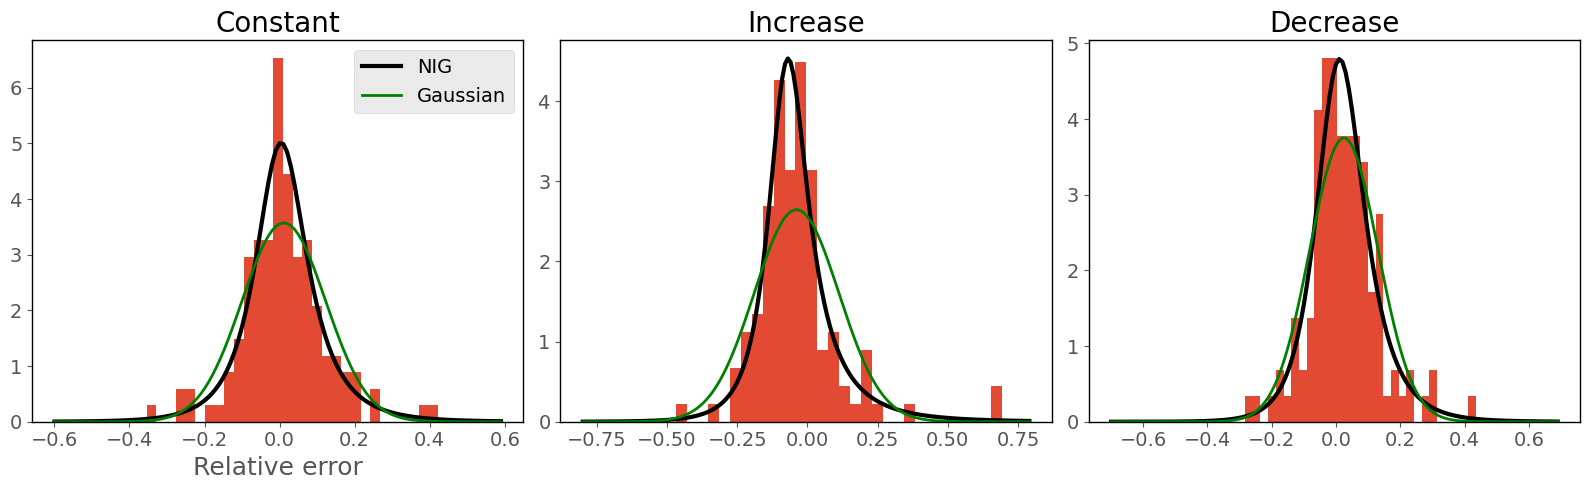}
    \caption{Same as Fig. \ref{fig:dist_zucchini} for the tomato series. }
    \label{fig:dist_tomato}
\end{figure}

\begin{figure}[!ht]
    \centering
    \includegraphics[width=1.0\textwidth]{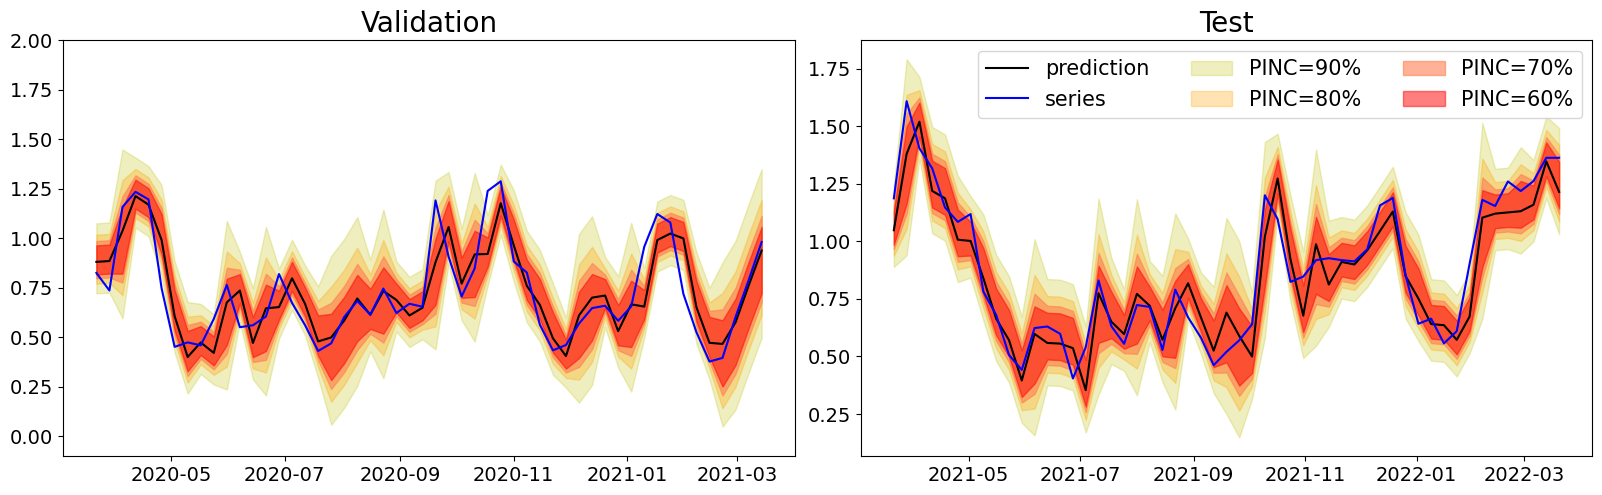}
    \caption{Predicted confidence interval for the tomato time series for the validation and test set.}
    \label{fig:intervals_tomato}
\end{figure}

\begin{table}[!ht]
    \centering
    \begin{tabular}{cccccccc}
    \hline \hline\\[-0.3cm]
                      &  \multicolumn{6}{c}{ \textbf{T O M A T O}} &\\
                        \cmidrule(lr){2-4}\cmidrule(lr){5-7}
                       \cmidrule(lr){2-7}
                      & & \multicolumn{3}{c}{Validation} &  \multicolumn{3}{c}{Test}\\
                        \cmidrule(lr){3-5}\cmidrule(lr){6-8}
        %\hline
         PINC  & Distribution   & PICP & ACE & PIAW & PICP & ACE & PIAW\\
        \hline \\[-0.3cm]
        \multirow{ 2}{*}{90\%} & NIG & 0.904 & 0.0038   & 0.537 & 0.962 & 0.062 & 0.492 \\
        & Gaussian & 0.885 & -0.015 & 0.512 & 1.0& 0.1 & 0.481 \\
        \hline \\[-0.3cm]
        \multirow{ 2}{*}{80\%} & NIG   & 0.769 & -0.0307 & 0.374   & 0.905 & 0.105 & 0.346 \\
        & Gaussian &  0.846 & 0.046 & 0.399 & 0.925 & 0.124 & 0.374\\
        \hline \\[-0.3cm]
        \multirow{ 2}{*}{70\%} & NIG  & 0.673 & -0.027 & 0.284   & 0.698   & -0.002 & 0.263 \\
        & Gaussian & 0.788 & 0.088& 0.323 & 0.792 & 0.092 & 0.303\\
        \hline \\[-0.3cm]
        \multirow{ 2}{*}{60\%} & NIG & 0.596 & -0.004 & 0.220   & 0.622   & 0.023 & 0.205 \\
        & Gaussian & 0.673 & 0.073 & 0.262 & 0.755 & 0.155 & 0.246\\
         \hline
    \end{tabular}
    \caption{Same as Table \ref{tab:intervals_zucchini} for the tomato time series.}
    \label{tab:intervals_tomato}
\end{table}

In summary, this section presents a method for estimating confidence intervals of the RC model by examining the statistical distribution of prediction errors. The analysis reveals that the NIG distribution is the most appropriate for modeling the error distribution in the case of the three vegetables studied. In contrast, the Gaussian distribution tends to overestimate the width of the confidence intervals, making the NIG distribution a superior choice.

%%%%%%%%%%%%%%%%%%%%%%%%%%%%%%%%%%%%%%%%%%%%%%%%%%%%%%%%%
% RESERVOIR COMPUTING PEPPER'S NETWORK
%%%%%%%%%%%%%%%%%%%%%%%%%%%%%%%%%%%%%%%%%%%%%%%%%%%%%%%%%

\section{Reservoir computing for cross-correlated forecasting }
\label{paper:RC_pimientos}

In the previous section, we developed and validated the optimal RC-based model to forecast food markets. The algorithm was used to predict the time evolution of three different products (zucchini, aubergine and tomato) independently. In that setting, the three studied products were significantly different, so that the price of one product did not influence the prices of the other ones.

\begin{figure}[!ht]
    \centering
    \includegraphics[width=0.5\textwidth]{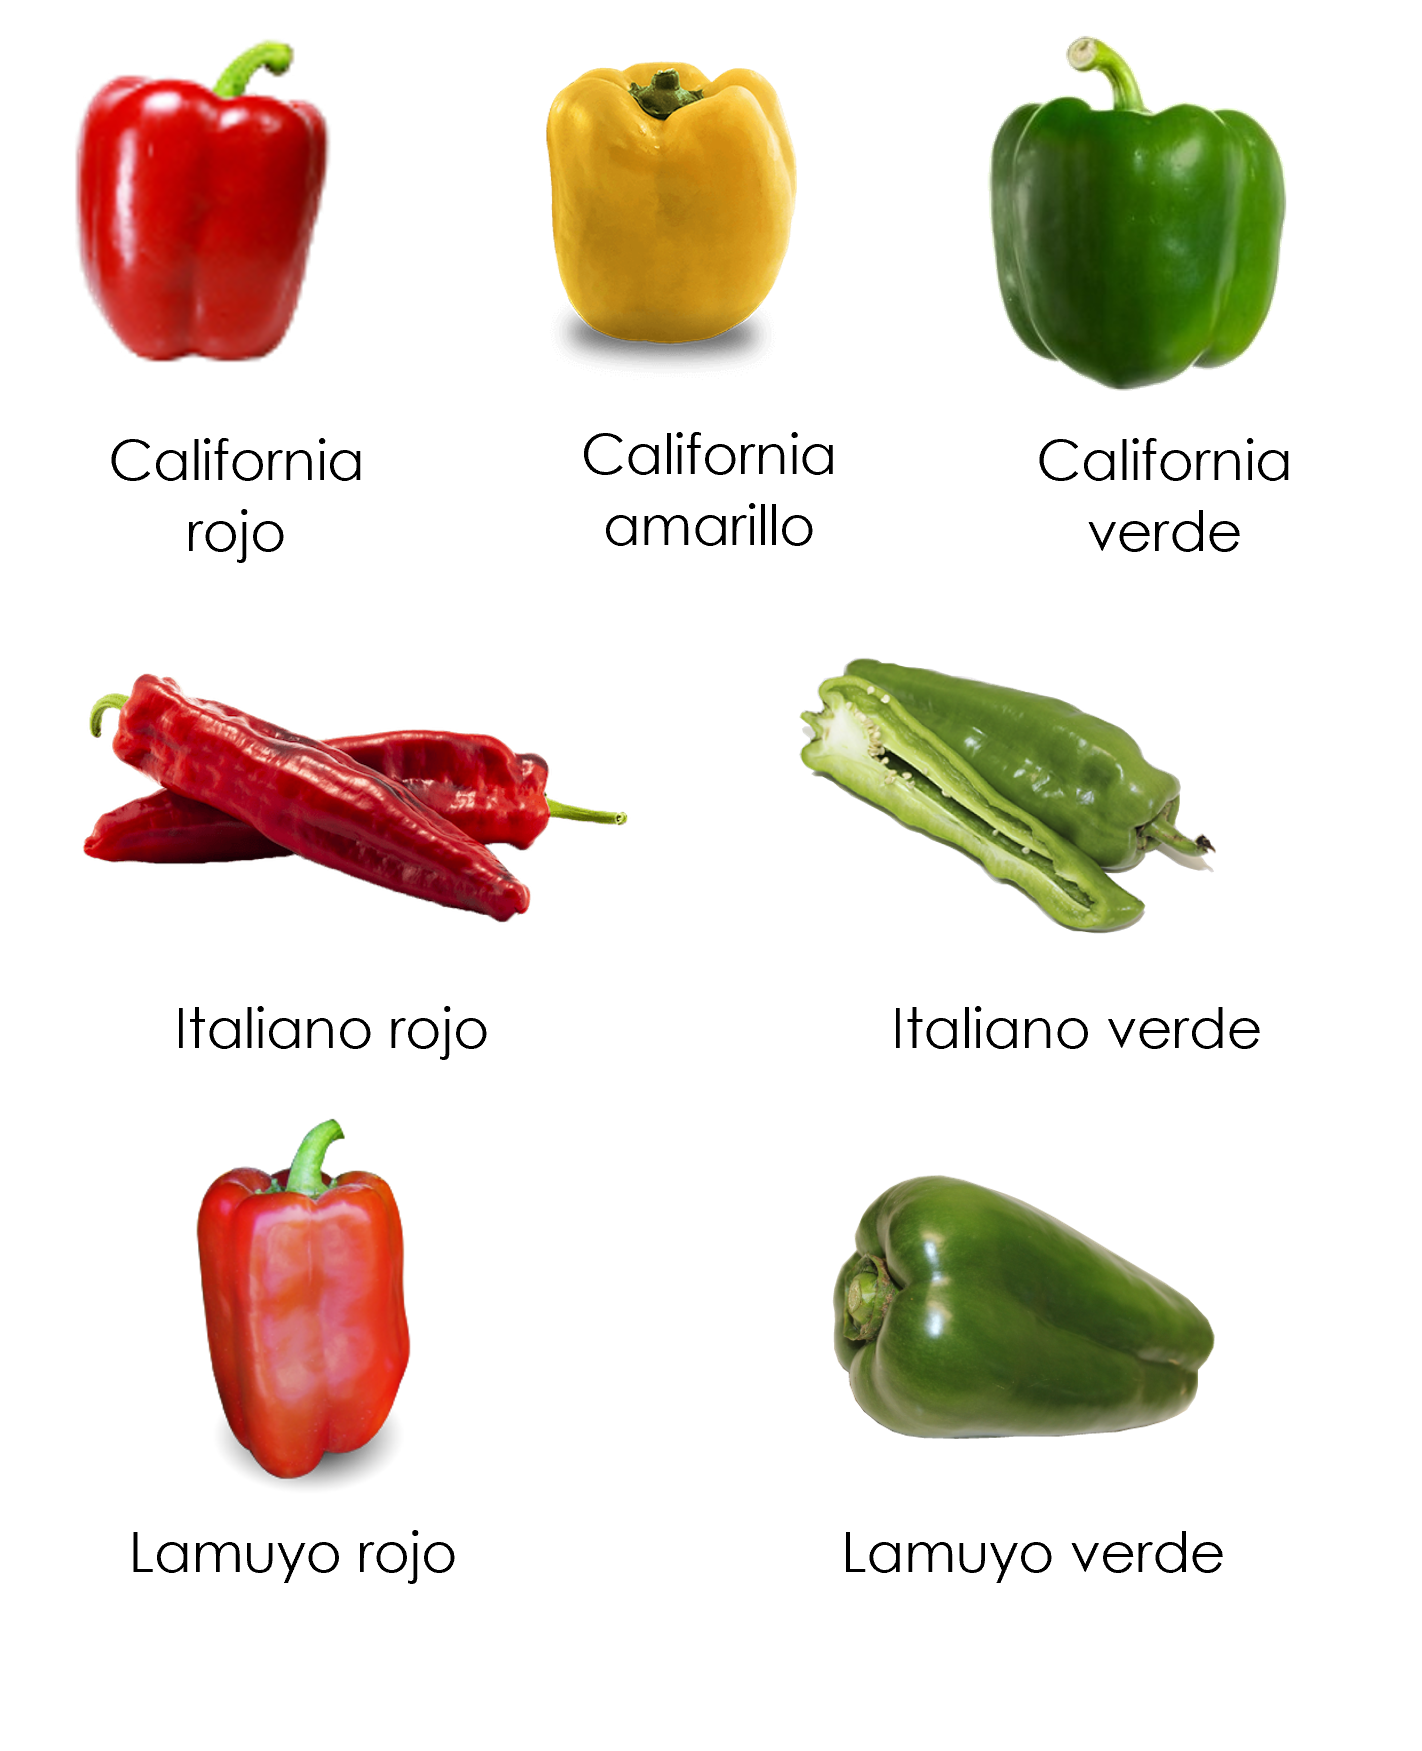}
    \caption{Names and images of the seven pepper varieties used for the cross-correlation forecasting analysis.}
    \label{fig:all_peppers}
\end{figure}
However, when studying the prices time evolution of similar products, the series may present a positive or negative correlation with each other. In these situations, it is important to study the cross-correlation when forecasting future prices, as incorporating the correlation information may improve the accuracy of the predictions. For example, different types of peppers such as green, yellow and red peppers may have positively correlated prices as they are often bought and offered together by grocery stores. On the other hand, similar products, such as different varieties of green peppers, may have negatively correlated prices as consumers tend to purchase only one type of them.

\begin{figure}[!ht]
    \centering
    \includegraphics[width=1.05\textwidth]{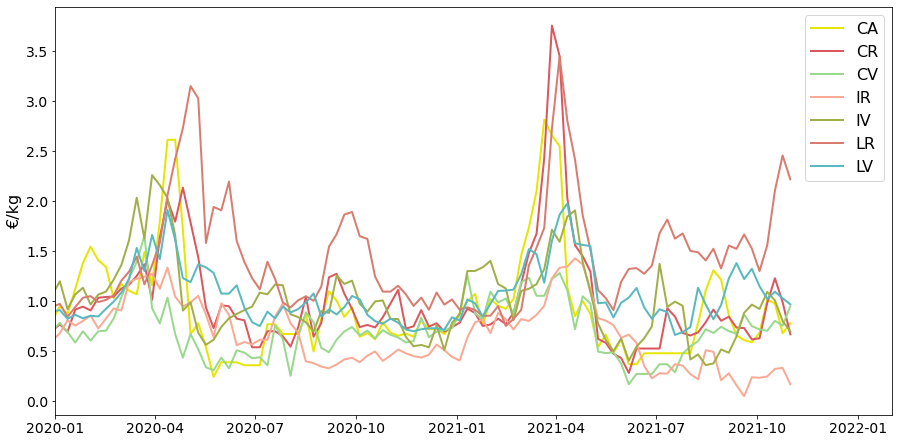}
    \caption{Time evolution of the prices per kilogram of the seven peppers types used in this work, during the years 2020-2021.}
    \label{fig:peppers_series}
\end{figure}
In this section, we explore how to design a multivariate forecasting model based on RC, so that the price evolution of multiple products is modeled simultaneously, taking into account their interdependencies. For this analysis, the weekly prices, again in euros per kilogram, of various types of peppers from the southeast region of Spain are used as the time series data. The seven varieties of peppers, which are shown in Fig. \ref{fig:all_peppers}, are denoted by their Spanish name: \emph{California Rojo} (\gls{CR}), \emph{California Amarillo} (\gls{CA}), \emph{California Verde} (\gls{CV}), \emph{Italiano Verde} (\gls{IV}), \emph{Italiano Rojo} (\gls{IR}), \emph{Lamuyo Rojo} (\gls{LR}) and \emph{Lamuyo Verde} (\gls{LV}). Our dataset includes prices from 2013 to 2021, and their evolution during the years 2020-2021 is depicted in Fig. \ref{fig:peppers_series}. The training set contains the samples from 2013 to 2019 (364 data points), the validation set contains the data from 2020 (52 data samples) and the test set contains the data from 2021 (43 data points). Also, 31 regressor variables, containing information about production volumes and international trade, are used as input to the RC models.

In the following sections, we will compare the performance of RC in predicting each of the time series independently, with the performance of RC models which take into account the correlation between the time series. The results show that a single joint model that predicts all the time series at the same time does not produce better results than the individual models. The reason for this is that the joint model's task is seven times more complex than the individual models' task, while the number of training samples is the same. For this reason, the joint RC model is likely to produce overfitting and thus is unable to correctly generalize to unseen observations. However, the linear cross-correlation analysis of the time series reveals that there are time-delayed correlations between the prices of different peppers. This indicates that past values of some time series can be used to predict the future evolution of other series. With this information we construct a cross-correlation network used to enhance the performance of the individual RC models by incorporating the past prices of carefully selected products as regressor variables. For simplicity, the joint and individual models are first evaluated by using the E-RC algorithm (See Sect. \ref{subsec:B}), since it requires training and optimizing only one ML model for each time series. After drawing conclusions from this analysis, the calculation is repeated using the D-RC algorithm (see Sect. \ref{subsec:C}), which proved to give optimal performance in the previous work. The resulting conslusions are the same as the ones from the E-RC method.

\subsection{Individual reservoir computing models}

The first step of this analysis consists of training one E-RC model for each of the seven time series. Apart from using information of past values of the time series to make the predictions, 31 regressor variables are also provided to as input to the RC model. The names and meaning of the variables are not given here for data confidentiality reasons. Even though these variables can provide insightful information to improve the predictions, they also increase the complexity of the ML model. ML models with more training parameters are more likely to overfit the training data and have poor generalization capacity. Moreover, we aim to design joint models which use information from other series as predictor variables, causing the number of variables to increase even more. For this reason, it is of uttermost importance to minimize the number of variables given to the RC algorithm. 

The optimization of the number of variables is done by estimating the importance of each predictor for the RC performance. To do so, we have trained E-RC models allowing connections from the input layer (the regressor variables) to the output layer (the predictions). That is, the output connection has shape $W^{\text{out}}\in M(\mathbb{R})_{L\times K+N}$, where $W_{i,j}^\text{out}$ for $1 \leq j \leq K $ is the weight from the $j$-th input unit to the $i$-th output unit (see Sect. \ref{sect:RC}). Then, the absolute value of the coefficients of $W_{i,j}^\text{out}$ for $1 \leq j \leq K$ can be used as a measure of variable importance. Notice that this is only valid since the variables are standarized to be in the $[-1,1]$ set. An example of the importance coefficients for the IV series is given in Fig. \ref{fig:var_importance} (a). The red-shadowed regions represent variables which have high importance coefficients, either being positively or negatively correlated with the target series. The variables in the yellow-shadowed areas have lower, but possibly relevant, importance, while the non-shadowed areas have importance closer to zero. 

\begin{figure}[!ht]
    \centering
    \includegraphics[width=0.85\textwidth]{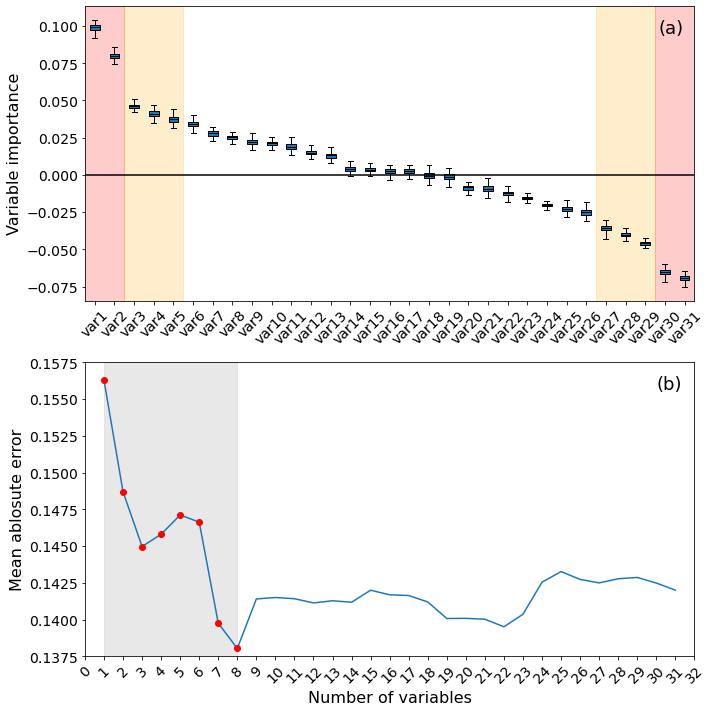}
    \caption{(a) Variable importance of the RC model for the IV time series. (b) Mean absolute error of the predictions obtained with the RC model for different number of regressor variables, ordered according to increasing variable importance.  }
    \label{fig:var_importance}
\end{figure}

To select the optimal number of variables, we use the importance coefficient to sort the variables in decreasing order, so that the first variable has the highest importance and the last variable has the lowest importance. Then, the E-RC model (this time without input-output connections) is retrained for different number of predictor variables. That is, the first E-RC model will only use the most important variable (calculated as we explained before), the second E-RC model will use the two most important variables, and so on. The MAE of the predictions in the test set for all these E-RC models is shown in Fig. \ref{fig:var_importance} (b). As can be seen in the figure, the MAE decreases with the number of variables for the first 8 E-RC models (see the shaded region). Then, the performance of the following E-RC models oscillates around MAE$=0.14$. Thus, we conclude that only 8 variables are enough to obtain optimal performance for the E-RC model in the IV series. This analysis is repeated for the other six time series. The optimal number of variables used by the E-Rc models, for each time series, is given in Table \ref{tab:optimal_num_vars}. 
\begin{table}
    \centering
    \begin{tabular}{c|ccccccc}
    \hline\hline \\[-0.3cm]
        Model & IV & IR & LV & LR & CV & CR & CA \\
        \hline \\[-0.2cm]
        Number of variables & 8 & 9 & 16 & 13 & 6 & 17 & 9 \\
        \hline
    \end{tabular}
    \caption{Optimal number of regressor variables used to train the individual reservoir computing models for the seven time series at study.}
    \label{tab:optimal_num_vars}
\end{table}

\begin{table}[!t]
    \centering
    \begin{tabular}{c|cccccc}
    \hline\hline \\[-0.3cm]
          Time series & $\alpha$ & $N$ & $\gamma$ & $\rho(W)$ & $D(W)$ & $N_e$  \\
          \hline \\[-0.2cm]
         IV & 0.72 & 140 & 1.5 & 1.14 & 0.025 & 140 \\
         IR & 0.91 & 240 & 2.9 & 1.1 & 0.021 & 180 \\
         LV & 0.68 & 200 & 0.51 & 0.88 & 0.016 & 140 \\
         LR & 0.71 & 80 & 0.15 & 0.85 & 0.025 & 160 \\
         CV & 0.78 & 140 & 3.0 & 1.4 & 0.029 & 120 \\
         CR & 0.72 & 120 & 0.3 & 1.2 & 0.024 & 260\\
         CA & 0.71 & 200 & 0.2 & 1.3 & 0.021 & 180 \\
         Joint model & 0.9 & 300 & 2.9 & 0.74 & 0.015 & 200 \\
      \hline   
    \end{tabular}
    \caption{Optimal hyperparameters used to train the reservoir computing model for the seven time series and the joint model. $\alpha$ is the leaking rate, $N$ the number of neurons of the reservoir, $\gamma$ is the regularization parameter, $\rho(W)$ and $D(W)$ the spectral radius and density of $W$, and $N_e$ the number of reservoirs used in the ensemble.}
    \label{tab:params_separate_models}
\end{table}

Once the number of variables has been optimized, we test the performance of the individual RC models in the test set. This performance will be used to make a comparison with the multivariate RC models. Just as in Sect. \ref{paper:RC_calabacines}, a Bayesian optimization method is used to find the optimal training parameters for the individual models, which are given in Table \ref{tab:params_separate_models}. The MAE and MDA in the test set are shown in Fig. \ref{fig:separate_RC}. For all pepper varieties the MDA is higher than 0.4 and even higher than 0.67 for the IV series. Notice that this performance will be later improved by using the D-RC algorithm instead of the E-RC.

\begin{figure}[!ht]
    \centering
    \includegraphics[width=0.95\textwidth]{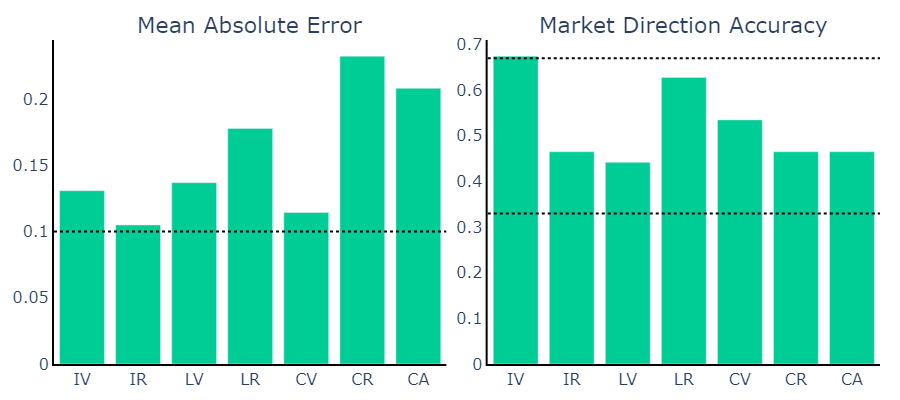}
    \caption{Mean absolute error and market direction accuracy for the individual reservoir computing models applied to the seven time series studied in this work in the test set.}
    \label{fig:separate_RC}
\end{figure}

\subsection{Joint reservoir computing model}
After obtaining the benchmark performance for the individual RC models, we design a joint RC model that predicts the evolution of the seven pepper time series at the same time. That is, the model takes as input all the regressor variables (78 in total) and the past value of the seven time series, and outputs a 7-dimensional vector containing the joint predictions. Since the reservoir has information of all the series and variables at the same time, it can potentially use the existing correlations and dependencies between series to improve the final predictions. However, notice that the complexity of the model has increased significantly, since instead of using 6-17 variables as input, it uses 78 variables. Moreover, the output has seven dimensions instead of one, which also increases the dimension of $W^\text{out}$. Models with higher complexity require more data samples to avoid overfitting the training set. In this case, the training size is kept constant, which poses a challenge for the RC model. The optimal parameters for the joint RC model are given in Table \ref{tab:params_separate_models}. Figure \ref{fig:joint_RC} shows the MAE and MDA of the predictions of the joint model in the test set, compared to the metrics of the individual RC models.

As can be seen, the joint RC model does not present a significant advantage over the individual RC models. For some pepper varieties, such as the IV, the performance of the joint RC model is worse than the individual RC predictions. For other types of peppers, such as the IR, the joint model has slightly lower MAE and higher MDA, improving the performance of the individual RC model. Therefore, we conclude that the joint model provides equivalent, or even slightly worse performance than the individual RC models, thus not representing any advantage. We believe that the main reason for this is the increased complexity of the joint model, which affects its generalization capacity. In the next section we show that predicting the seven series at the same time, without using the correlations between series, does decrease the predicting capacity, confirming this hypothesis.

\begin{figure}[!ht]
    \centering
    \includegraphics[width=0.95\textwidth]{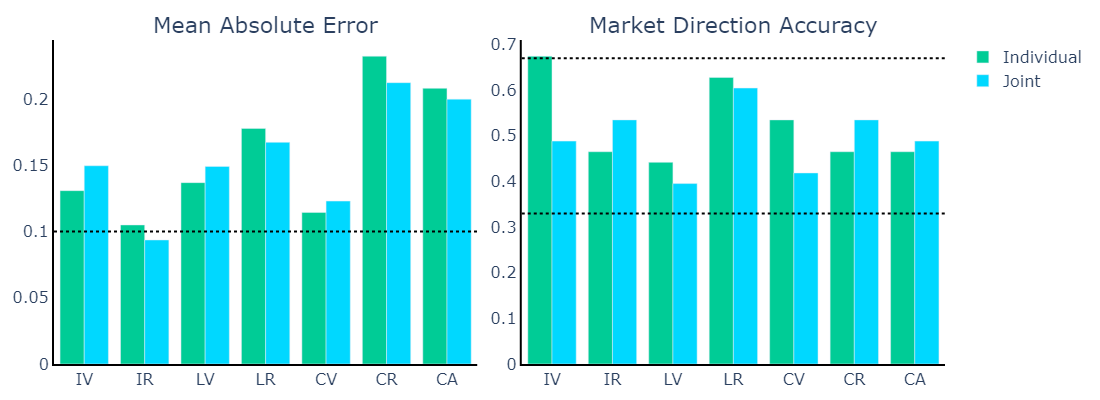}
    \caption{Mean absolute error and market direction accuracy for the joint reservoir computing model which predicts the prices of the seven products simultaneously in the test set, compared to the performance of the individual RC models.}
    \label{fig:joint_RC}
\end{figure}

\subsection{Joint model with block-diagonal matrices}
In this section, we create a joint RC model that uses all 78 variables and processes all seven series simultaneously. However, the model is not allowed to use correlations between the time series. The purpose of this design is to demonstrate that the increased complexity of the joint RC model is the primary reason for the lack of improvement in predictions. With it, we aim to show that accounting for the correlation between series should enhance the final predictions, but the high dimensionality of the learning algorithm hinders this effect.

In order to prohibit the model from considering correlations between series, the matrices of the RC algorithm are chosen to be block-diagonal, so that the internal state of the network $x(t)$ is a concatenation of internal states $x_i(t)$, each using information of the individual time series. That is,

\begin{equation}
    x(t) = 
    \begin{pmatrix}
    x_1(t)\\
    x_2(t)\\
    \vdots \\
    x_7(t)
    \end{pmatrix}, \quad 
    W^k = \begin{pmatrix}
        W_1^k & 0& 0 & \cdots & 0\\
        0 & W_2^k & 0 & \cdots & 0\\
        \vdots & &\cdots & & \vdots \\
        0 & 0 & \cdots & 0 & W_7^k
    \end{pmatrix}, \quad W^k \in \{W, W^\text{in}, W^\text{out}\}
\end{equation}
with $W_i \in M(\mathbb{R})_{N/7\times 1}$, $W_i^\text{in} \in M(\mathbb{R})_{N/7\times K_i}$ and $W_i^\text{out} \in M(\mathbb{R})_{1\times K_i+N/7}$ for $i \in \{1, \cdots, 7\}$. We refer to this RC model as block-diagonal RC, since the internal matrices are forced to be block-diagonal. The performance of this model in the test set is shown in Fig. \ref{fig:block_diagonal}, compared to the performance of the joint model, described in the previous section.

As can be seen, the block-diagonal RC clearly has worse performance than the joint RC, both in terms of MAE and in terms of MDA. The difference between these two RC models is that the joint RC is allowed to consider the correlations between variables and series, while the block-diagonal RC is not. Thus, the results in Fig. \ref{fig:block_diagonal} prove that using cross-correlations between pepper time series does improve the performance of RC. However, the increase of model complexity without increasing the training set decreases performance in unseen data, which results in the joint RC model not presenting an advantage over the individual RC models. Therefore, a RC model which uses the correlation between series without having too high complexity may improve the predictions of the individual models. 

\begin{figure}[!ht]
    \centering
    \includegraphics[width=0.95\textwidth]{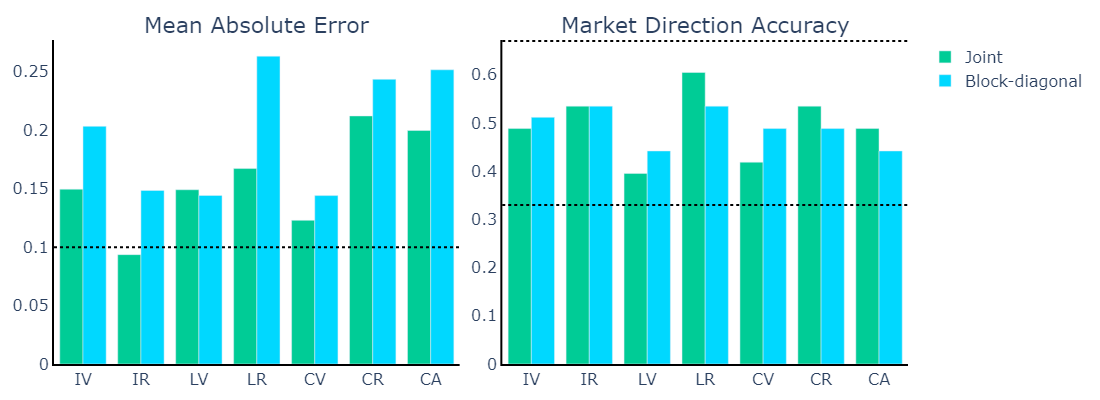}
    \caption{Mean absolute error and market direction accuracy for the block-diagonal reservoir computing model which predicts the prices of the seven products simultaneously in the test set, compared to the performance of the joint RC model.}
    \label{fig:block_diagonal}
\end{figure}

\subsection{Cross-correlation analysis}
In this section, we perform a linear cross-correlation analysis which allows us to identify the most relevant correlations between pepper time series. For this reason, we use the sample cross correlation function (\gls{CCF}), which is helpful for the description and modeling of the relationship between two time series $x_t$ and $y_t$. It measures the linear correlation between corresponding elements of two time series at different time lags. That is, the CCF helps identify which lags $h \in \{0, \pm 1, \pm 2, \cdots \pm N\}$ of $x_{t+h}$ are useful to predict $y_t$. Mathematically,
\begin{equation}
    CCF(h) = \frac{\sum_{t=1}^{n-h} (x_t - \bar{x})(y_{t+h} - \bar{y})}{\sqrt{\sum_{t=1}^{n-h} (x_t - \bar{x})^2 \sum_{t=1}^{n-h} (y_{t+h} - \bar{y})^2}},
\end{equation}
where $\bar{x}, \bar{y}$ are the means of the respective time series, and 
$h$ represents the time lag.
\begin{figure}[!ht]
    \centering
    \includegraphics[width=0.75\textwidth]{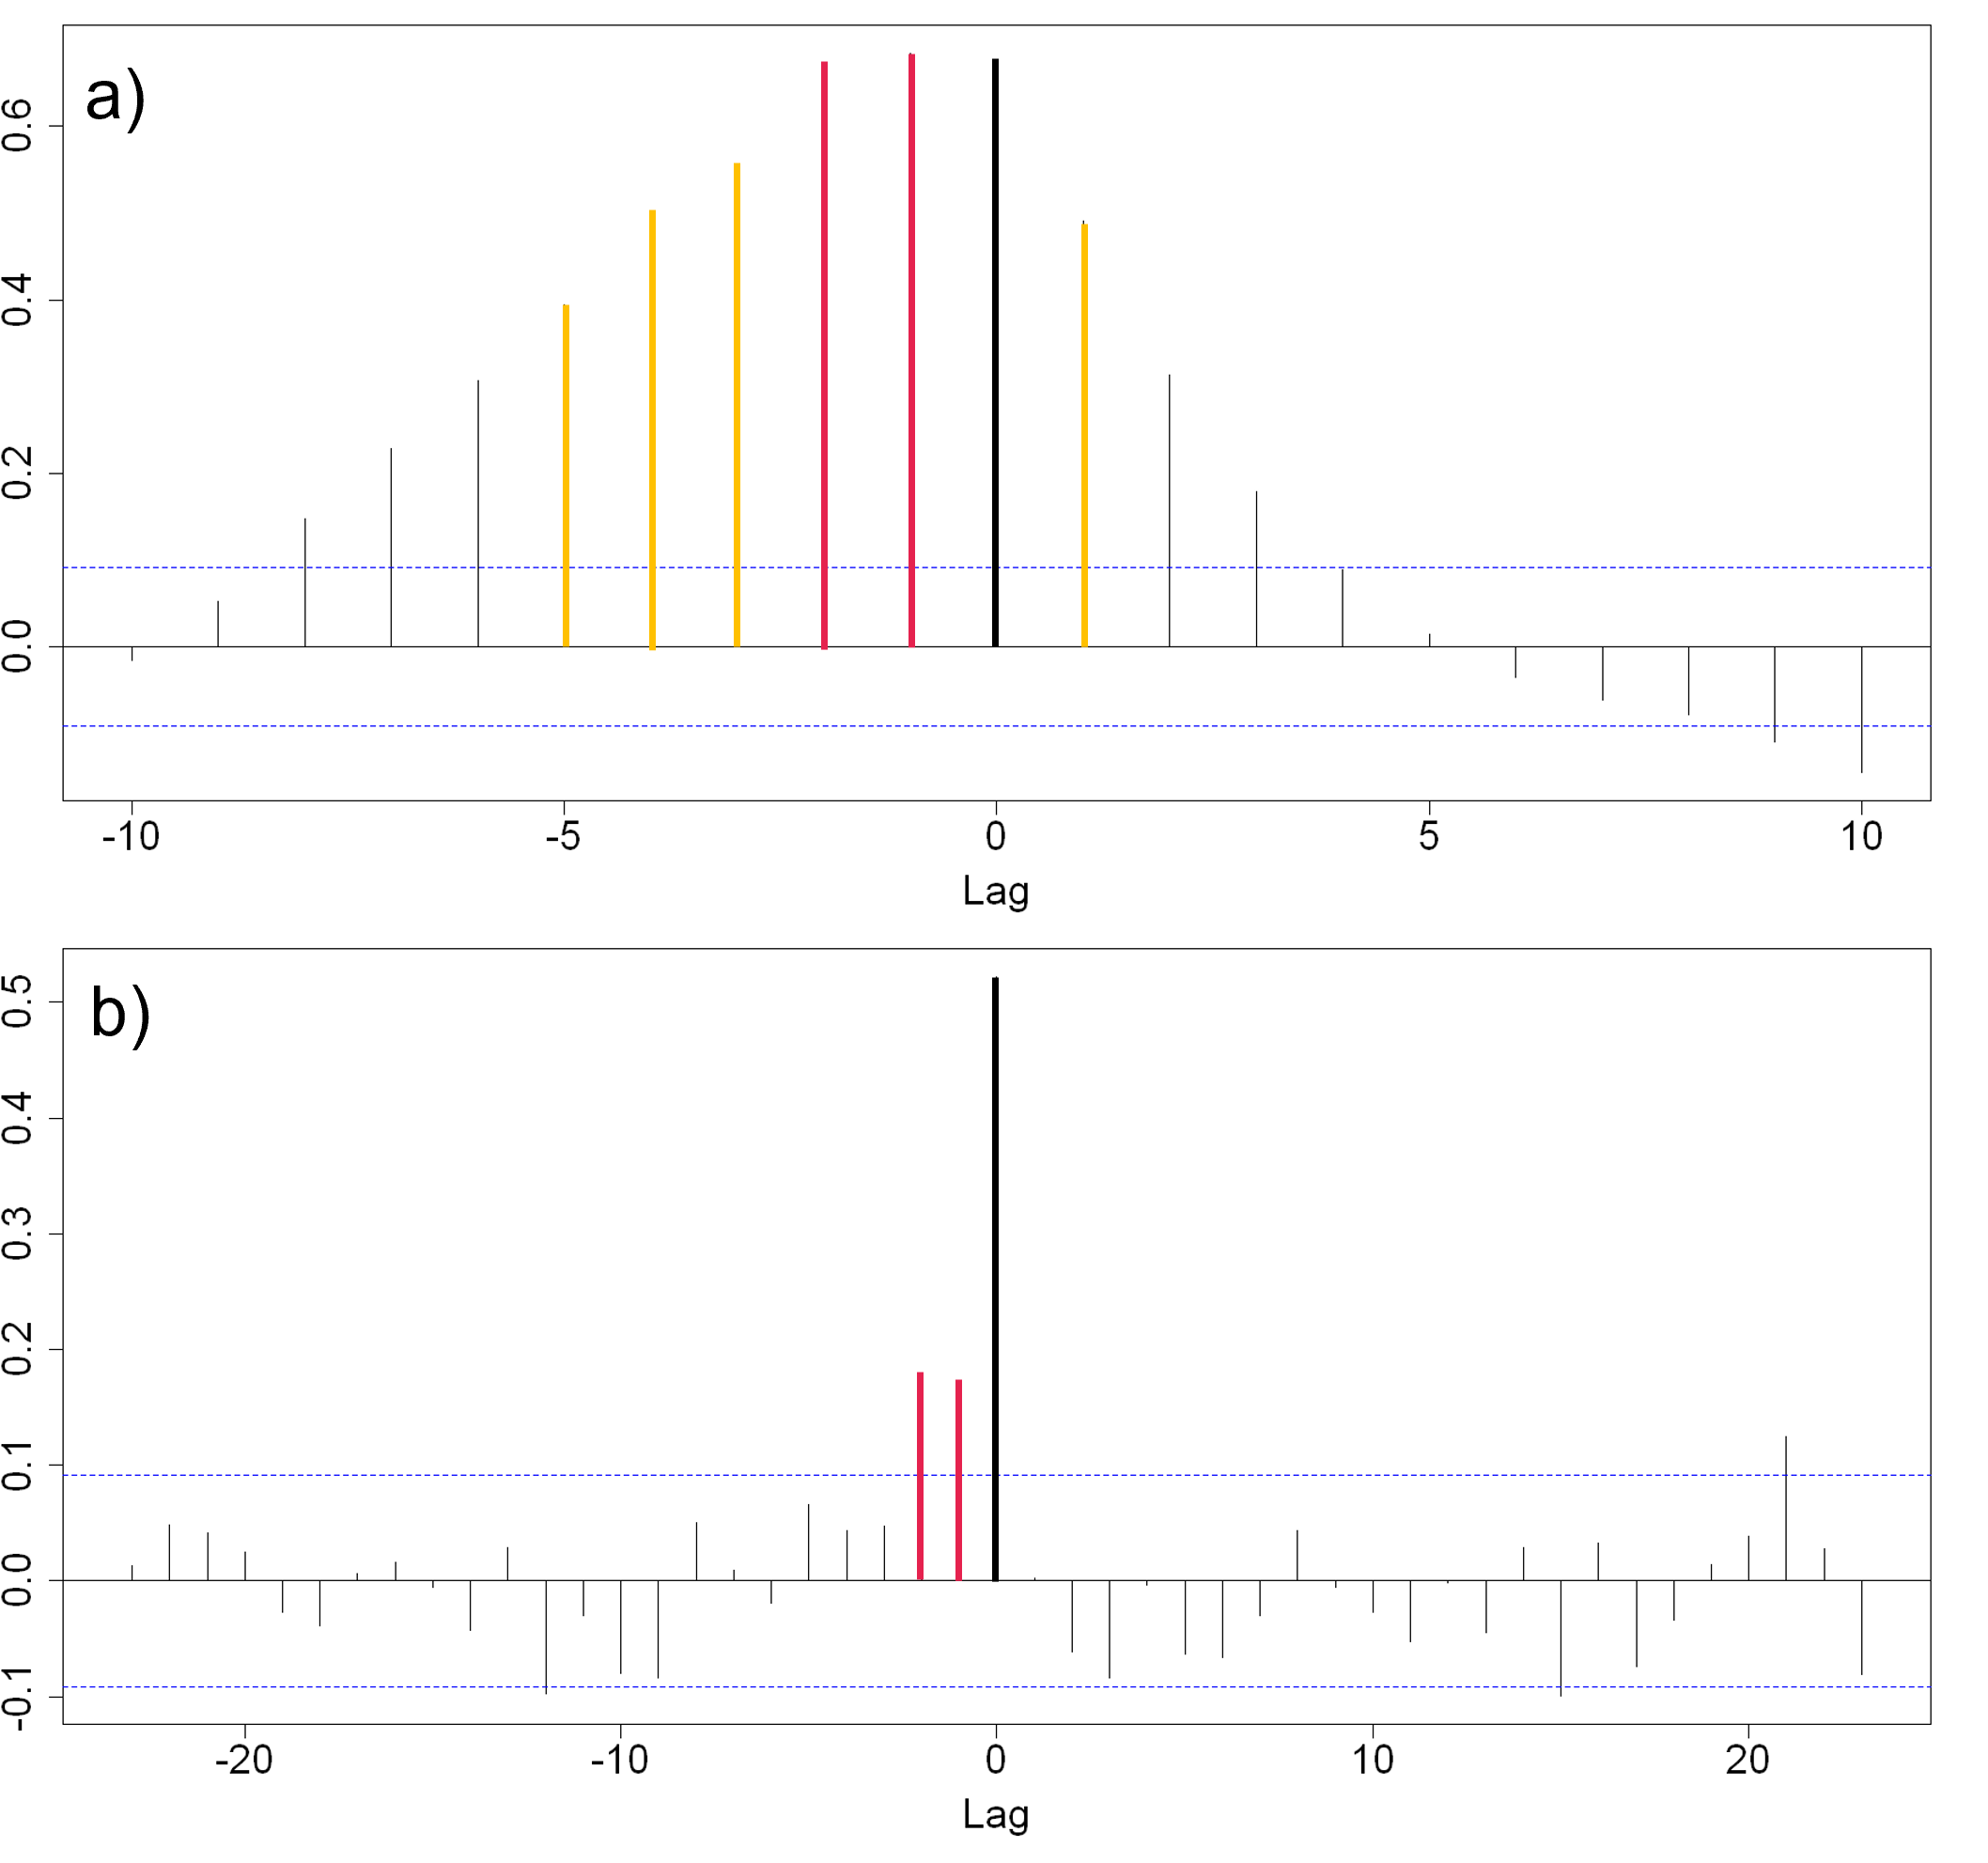}
    \caption{a) Cross-correlation function for the CA and CR time series. b) Cross-correlation function for the pre-whitened  CA and CR time series. The highlighted black lines show the cross-correlation at lag 0, the red lines mark the lags with statistical significant correlation in both the original and pre-whitened series, and the yellow lines mark the sinusoidal behavior of the cross-correlation function.}
    \label{fig:cross-correlation}
\end{figure}

If there are significant high peaks in the CCF for negatives values of $h$, then past values of the series $x_t$ may be useful to predict the future of $y_t$. On the other hand, if there are peaks in positive values of $h$, then past values of $y_t$ may help predict future values of $x_t$. Figure \ref{fig:cross-correlation} a) shows an example of the CCF for the $x_t = CA$ and $y_t=CR$ time series. We see that there are significant peaks at lags different from zero (marked in red), $h=-1, -2$, and then the CCF decays in a sinusoidal manner (marked in yellow). This suggest that there is a dependency around $h=-1,-2$, so that the values $x_{t-1}$, $x_{t-2}$ could be useful to predict $y_t$. The sinusoidal decay also suggests a dependency of $y_{t-1}$ and $y_{t-2}$. Notice that there is also a significant peak at lag 0 (highlighted in black), which indicates that the values $x_{t}$ could be useful to predict $y_t$. However, this result does not provide useful information for our task, since the values of $x_t$ are not available when making the predictions of $y_t$.

The CCF is a relevant tool to detect time-delayed correlations. However, the CCF is affected by the time series structure of $x_t$ and any in common trends the $x_t$ and $y_t$ series may have over time. For this reason, it is essential to remove the trends and seasonal patterns from both series before analyzing the associated CCF. Such strategy is called pre-whitening the time series. The first step consists of determining a time series model using SARIMA for $x_t$ and store the residuals from such model. Then, the $y_t$ series are filtered with the $x_t$ SARIMA model (using the estimated coefficients from the previous step), obtaining the residuals of $y_t$ based on the $x_t$ model. With this process, all the temporal patterns present in the series $x_t$ are removed, and the correlation between the two series can be properly assessed, by examining the CCF between the $x_t$ residuals and the filtered $y_t$ values. Notice that it is not necessary to find an exact model for the $x_t$ series (which probably does not exist), but just to remove strong temporal patterns. 

With this analysis we observe that there are in fact time-delayed correlations between the seven time series. Figure \ref{fig:cross-correlation} b) shows the CCF for the CA and CR pre-whitened series. The sinusoidal pattern has now disappeared, since it was caused by the dependencies of the past values of the same series. However, we do observe two significant peaks at lags $h=-1,-2$, which means that the values of $x_{t-1}$, $x_{t-2}$ from the CA series could be useful to predict $y_t$ for the CR series. This analysis is then repeated for each pair of time series, identifying the cross-correlation between the series that can possibly be used to improve the predictions of the RC model. With this information, we build a network, where the nodes represent each of the seven time series, and a directed link between two nodes is added if a past values of the origin node may be useful to predict the future of the destiny node, based on the cross-correlation analysis. The weights of the links correspond to the lags $h$ which present significant cross-correlation. Notice that the sign of the lag is encoded in the direction of the link. The resulting network is shown in Fig. \ref{fig:networks_peppers} a). All the significant cross-correlations appear in small values of $h$, since the link weights are no bigger than 4. This means that the time-delayed correlations do not last longer than four weeks, which agrees with the high volatility of the series.

\begin{figure}[!ht]
    \centering
\includegraphics[width=1.1\textwidth]{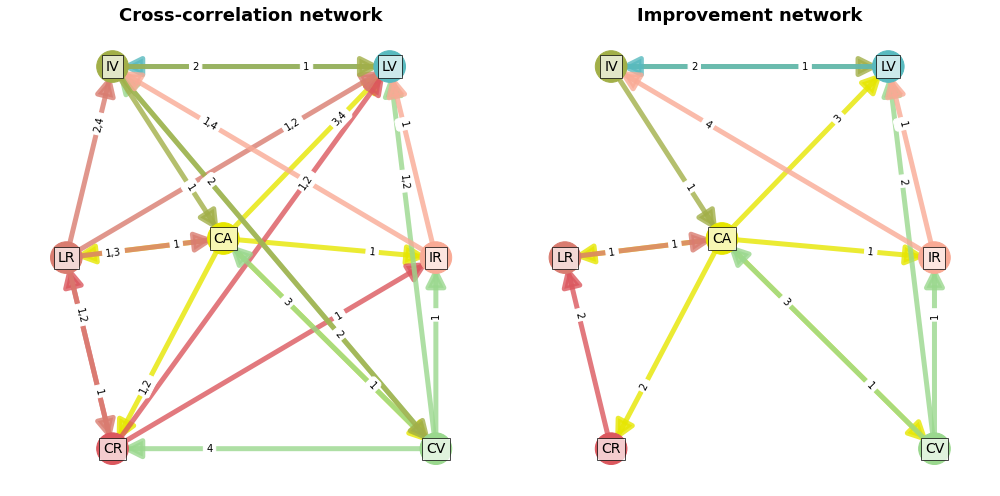}
    \caption{a) Cross-correlation network. The nodes correspond to the prices time series of the seven varieties of peppers. A directed link appears if there is a time-delayed correlation between the two time series, so that past values of the origin node are correlated with future values of the destiny node. The weights of the links represent the correlated time delays. b) Performance improvement network. A link from a node to another means that the time-delayed series of the origin node improves the prediction of the destiny node.}
    \label{fig:networks_peppers}
\end{figure}

\subsection{Individual models with cross-correlated variables}
In this section, we use the cross-correlation network developed in the previous section (Fig. \ref{fig:networks_peppers} a)) to enhance the performance of individual RC models. Indeed, the nodes connecting to a specific time series have the potential to improve the performance of the RC algorithm. However, since the network only captures pairwise correlations between series it may contain redundancies, as different series may provide the same information to the ML model. To address this issue, we aim to identify the smallest set of time-delayed series (if any) that does improve the performance of RC. 

To this end, we use the selected time-delayed series from the network as predictor variables for the target time series. Specifically, given a time series $y_t$ that we aim to forecast, we consider a node $x_t$ of the network which has a link with weight $h$ to the series $y_t$. Then, the $h$-time-delayed series of the $x_t$ series is used as an input variable to the RC algorithm, along with the other predictor variables of the $y_t$ series. In this way, a predictor variable is added for every neighbor and weight of the node $y_t$. To test which nodes connected to $y_t$ are needed to improve the RC performance, we evaluate the MAE in the validation set for all the combinations of predictor variables. For example, the IR pepper series is linked to the series $\{\text{CR}_1, \text{CA}_1, \text{CV}_1\}$ (see the network in Fig. \ref{fig:networks_peppers}), where $\text{CR}_1$ means the CR series with lag $h=-1$. In this case, we evaluate the RC performance using all the combinations of these three elements: $\{\{\}, \{\text{CR}_1\}, \{\text{CA}_1\}, \{\text{CV}_1\}, \{\text{CR}_1, \text{CA}_1\}, \{\text{CR}_1, \text{CV}_1\}, \{\text{CA}_1, \text{CV}_1\}, \{\text{CR}_1, \text{CA}_1, \text{CV}_1\}\}$. In this way, the set of time-series that produces higher performance in the validation set forms the optimal set of predictor variables. This process is then repeated for each time series. With this information, the performance improvement network is built, and it is shown in Fig. \ref{fig:networks_peppers} b), where the nodes are linked only if the time-delayed series improved the performance of the RC algorithm. Notice that the number of links and weights is significantly smaller than before. This confirms the hypothesis that there were redundant links in the cross-correlation network. 
\begin{figure}[!ht]
    \centering
    \includegraphics[width=1.0\textwidth]{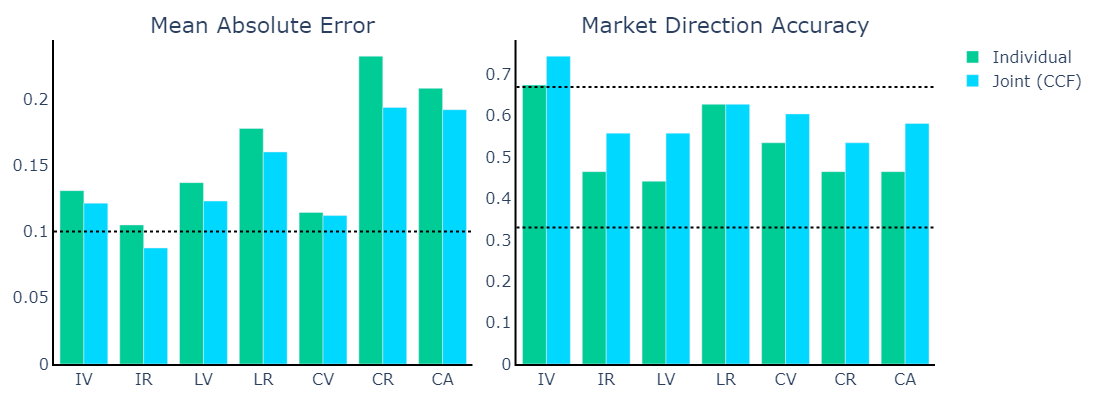}
    \caption{Mean absolute error and market direction accuracy for the individual reservoir computing models which use the cross-correlation analysis, applied to the seven time series studied in this work in the test set.}
    \label{fig:separate_CCF}
\end{figure}

Once we have identified the optimal set of extra regressor variables, we have to test whether the performance of the RC models in the test set is actually better than the performance of the individual RC models. The results are shown in Fig. \ref{fig:separate_CCF}. As can be seen, the MAE of all the pepper varieties for the RC model with cross-correlated variables is smaller than the MAE for the individual RC models. Moreover, the MDA of all the series is higher when using the cross-correlated variables. These results confirm the usefulness of the performance optimization network and the cross-correlation analysis. Moreover, this methodology does not only apply to the agri-commodities market, but it is useful for any dataset containing cross-correlated time series. 
\begin{figure}[!ht]
    \centering
    \includegraphics[width=1.0\textwidth]{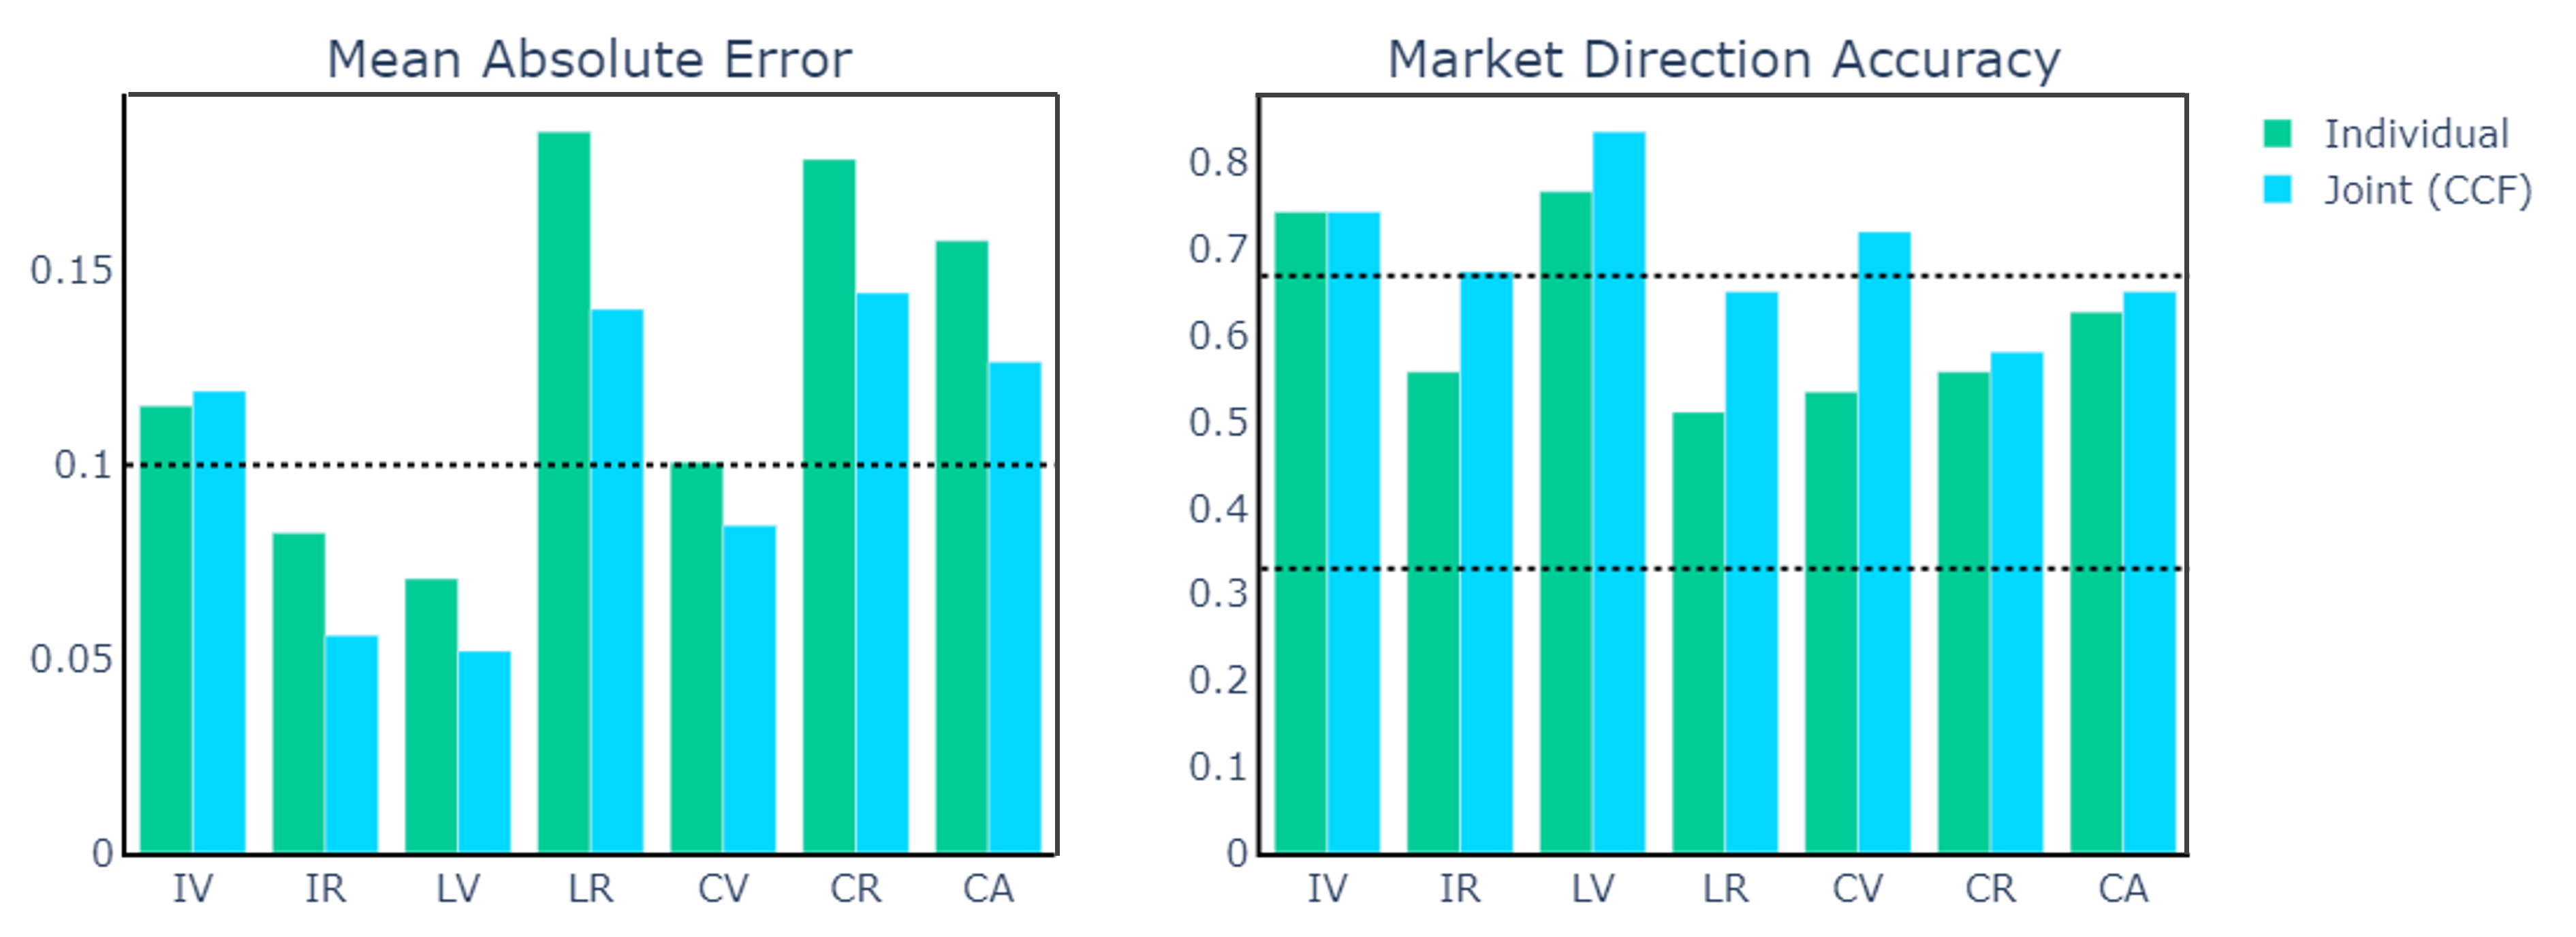}
    \caption{Mean absolute error and market direction accuracy for the individual decomposition reservoir computing (D-RC) models which use the cross-correlation analysis, applied to the seven time series studied in this work.}
    \label{fig:separate_CCF_dec}
\end{figure}

\subsection{Results with D-RC}

Until now, the E-RC algorithm has been used to train all the models, since the E-RC only requires optimizing one ML model for each time series. In this section, we check that the performance improvement network also improves the performance when using the D-RC algorithm, instead of the E-RC one. To this end, we train individual D-RC models for each pepper variety together with D-RC models using the performance improvement network to select additional predictor variables. The hyperparameters for the models, selected by Bayesian optimization, are given in Table \ref{tab:params_separate_models}. The performances of the D-RC models are shown in Fig. \ref{fig:separate_CCF_dec}. As can be seen, the D-RC models with cross-correlated variables provide better performance, both in terms of MAE and MDA, than the individual D-RC models. Therefore, we conclude that the cross-correlation analysis is also valid when using the D-RC algorithm.

\begin{table}[!t]
    \centering
    \begin{tabular}{c|cccccc}
    \hline\hline \\[-0.3cm]
          Time series & $\alpha$ & $N$ & $\gamma$ & $\rho(W)$ & $D(W)$ & $N_e$  \\
          \hline \\[-0.2cm]
         IV (trend) & 0.72 & 100 & 0.01 & 1.3 & 0.020 & 260 \\
         IV (seasonality) & 0.96 & 100 6 0.01 & 0.99 & 0.028 & 120\\
         IV (residuals) & 0.85 & 80 & 2.9 & 1.4 & 0.014 & 200\\[0.3cm]
         IR (trend) & 0.89 & 100 & 0.011 & 0.90 & 0.017 & 80 \\
         IR (seasonality) & 0.87 & 30 & 0.015 & 0.90 & 0.010 & 300 \\
         IR (residuals) & 0.68 & 120 & 3.0 & 0.57 & 0.019 & 180\\[0.3cm]
         LV (trend) & 0.77 & 100 & 0.012 & 1.2 & 0.019 & 40\\
         LV (seasonality) & 0.90 & 90 & 0.44 & 1.3 & 0.017 & 20\\
         LV (residuals) & 0.78 & 100 & 0.34 & 1.0 & 0.024 & 20\\[0.3cm]
         LR (trend) & 0.95 & 80 & 0.011 & 0.15 & 0.013 & 260\\
         LR (seasonality) & 0.73 & 20 & 0.012 & 1.3 & 0.018 & 120\\
         LR (residuals) & 0.88 & 30 & 2.11 & 0.80 & 0.012 & 120\\[0.3cm]
         CV (trend) & 0.77 & 80 & 0.013 & 0.74 & 0.022 & 220 \\
         CV (seasonality) & 0.87 & 90 & 0.015 & 1.1 & 0.016 & 220 \\
         CV (residuals) & 0.89 & 60 & 3.0 & 0.72 & 0.026 & 200\\[0.3cm]
         CR (trend) & 0.94 & 80 & 0.010 & 0.58 & 0.026 & 120\\
         CR (seasonality) & 0.70 & 80 & 0.010 & 0.93 & 0.024 & 240\\
         CR (residuals) & 0.85 & 60 & 3.0 & 0.72 & 0.025 & 200\\[0.3cm]
         CA (trend) & 0.93 & 80 & 0.010 & 0.58 & 0.026 & 120\\
         CA (seasonality) & 0.69 & 80 & 0.010 & 0.93 & 0.024 & 240\\
         CA (residuals) & 0.91 & 80 & 0.40 & 0.12 & 0.010 &120\\
      \hline   
    \end{tabular}
    \caption{Same as Table \ref{tab:params_separate_models} for the decomposition reservoir computing (D-RC) model.}
    \label{tab:params_separate_models}
\end{table}

All in all, the results presented here show that analyzing the cross-correlation between similar time series is key to designing optimal forecasting models. In this way, the time-delayed information from related products enhances the performance of the RC-based models. 

The time series studied here correspond to the agri-food market, whose accurate control is crucial to guarantee sustainability and reduce food waste. Forecasting these time series is very complicated since they contain very few data points, which poses a challenge when designing multivariate forecasting models, because of the increase of dimensionality of these models. Our approach minimizes the complexity of the resulting algorithm, while using the relevant interdependencies of the data. As a result, the applied methodologies are not restricted to agri-commodities predictions, but to any dataset containing substantially correlated series.
