# Supplementary material for: Classical and quantum reservoir computing: development and applications in machine learning
Source: arXiv:2310.07455 source file (2023-10-11)
Supplement: Supplementary file 2 [file appendix5.tex]

 %%%%%%%%%%%%%%%%%%%%%%%%%%%%%%%%%%%%%%%%%%%%%%%%%%%%%%%%%%%%%
 % QUANTUM COMPUTING
 %%%%%%%%%%%%%%%%%%%%%%%%%%%%%%%%%%%%%%%%%%%%%%%%%%%%%%%%%%%%%

\section{Quantum computing}
\label{sect:QC}
 Quantum mechanics is a mathematical framework used for the construction of physical theories. Quantum computing exploits the properties of quantum mechanics to perform information-processing tasks. The laws of quantum mechanics provide great computational power and are yet very different to the classical information rules. In this section, we introduce the terminology and fundamental concepts behind quantum mechanics (for a more detailed explanation see Ref. \citep{Nielsen}). Then, we introduce how this framework can be used to design quantum algorithms. In particular, we discuss the different trends in QML. Finally, we present the quantum algorithm that will be studied in this thesis, \gls{QRC}.

\subsection{The postulates of quantum mechanics}
\label{sect:postulates}
The postulates of quantum mechanics are in a fundamental sense the basis of any physical theory. They provide a connection between mathematical formalism and physical phenomena. For this reason, they set the rules for designing any QML algorithm. Each postulate defines a property of a quantum system. The first Postulate specifies how to describe the state of a quantum system while the second Postulate describes the time evolution of such system. Postulate 3 tells us how to extract information from a quantum system by performing measurements. Finally, Postulate 4 shows how states from different quantum systems can be combined to describe their composite state.

\begin{postulate}{1}
Associated with any closed physical system is a Hilbert space $\mathcal{H}$ known as the \emph{state space} of the system. The system is completely described by its \emph{state vector}, which is a unit vector in the system state space. Vectors that differ only by a global phase describe the same quantum state.
\end{postulate}

In general, it is not trivial to know the state space or state vector of a given physical system. The simplest physical system is the \emph{qubit}, whose state space is $\mathcal{H}_2 = \mathcal{C}^2$. The term qubit should not be confused with the term \emph{bit}, which refers to the fundamental unit of classical information. A bit has a state of either 0 or 1, while a qubit can have states $\ket{0}$, $\ket{1}$ or any \emph{superposition} (linear combination) of these two states. That is, the most general state of a qubit is 
\begin{equation}
    \ket{\psi} = a\ket{0}+b\ket{1}, \quad a,b \in \mathbb{C},
\end{equation}
where $\{\ket{0}, \ket{1}\}$ form a complete orthonormal basis of $\mathcal{H}_2$. The state $\ket{\psi}$ must be a unit vector, $\braket{\psi} =1$, which implies that the coefficients must fulfill $|a|^2 + |b|^2 = 1$. A useful geometric representation of single qubits states is the \emph{Bloch Sphere} representation, shown in Fig. \ref{fig:bloch_sphere}. A qubit can be represented as a point in the Bloch sphere by using two parameters $(\phi, \theta)$ in the following way 
\begin{equation}
    \ket{\psi} = \cos \frac{\theta}{2} \ket{0} + e^{i\phi} \sin \frac{\theta}{2} \ket{1}.
\end{equation}
\begin{figure}
    \centering
    \includegraphics[scale=0.8]{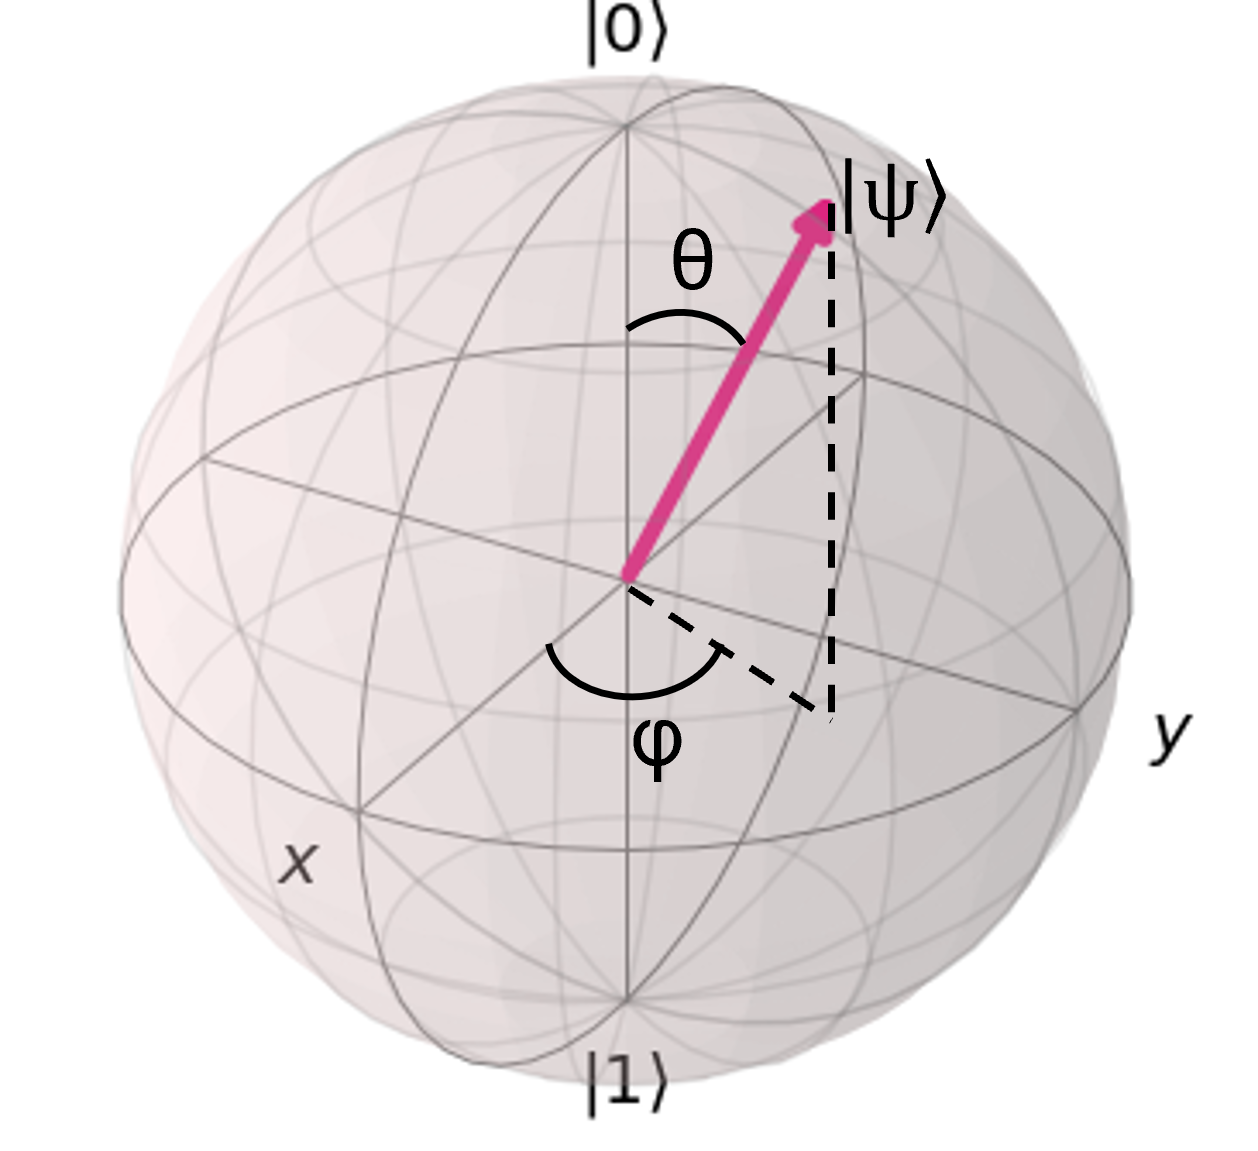}
    \caption{Bloch sphere standard representation.}
    \label{fig:bloch_sphere}
\end{figure}
A set of very useful operators that can transform one qubit state to any other qubit state are the \emph{Pauli matrices}. The matrix form of these operators is 
\begin{equation}
\mathbb{I} = \begin{pmatrix}
1 & 0\\
0 & 1
\end{pmatrix},\quad
    X = \begin{pmatrix}
    0 & 1 \\
    1 & 0
    \end{pmatrix}, \quad
    Y = \begin{pmatrix}
    0 & -i \\
    i & 0
    \end{pmatrix},\quad
    Z = \begin{pmatrix}
    1 & 0 \\
    0 & -1
    \end{pmatrix}.
    \label{eq:Pauli_matrices}
\end{equation}
These matrices make transformations between qubits.  $X$ transforms the state $\ket{\psi} = a\ket{0} + b\ket{1}$ to $a\ket{1} + b\ket{0}$, $Y$ transforms $\ket{\psi}$ to $-ia\ket{1} + ib \ket{0}$, $Z$ transforms $\ket{\psi}$ to $a\ket{0} - b\ket{1}$ and $\mathbb{I}$ leaves $\ket{\psi}$ unchanged. Moreover, it turns out that any one qubit state $\ket{\psi}$ can be written as a combination of the Pauli operators
\begin{equation}
    \ketbra{\psi} = \frac{\mathbb{I} + r_x X + r_y Y + r_z Z}{2}, \quad ||(r_x, r_y, r_z)|| = 1.
    \label{eq:pure_state_Pauli_decomposition}
\end{equation}
The following postulate describes the evolution of a state in time.

\begin{postulate}{2}
The evolution of a closed quantum system is unitary. That is, if the quantum state of a closed system is $\ket{\psi}$ at time $t$ and $\ket{\psi'}$ at time $t'$, then there exists a unitary operator $U$, which depends only on $t' - t$, such that
\begin{equation}
    \ket{\psi'} = U \ket{\psi}.
\end{equation}
\end{postulate}
Notice that the laws of quantum mechanics do not specify what unitary operators describe the dynamics of a particular quantum system, and it is the physicist's job to figure out this description. Moreover, Postulate 2 requires the quantum system to be closed so that it does not interact with any other system. In fact, there are no closed systems, except for the whole universe, but many systems can be approximately described as closed systems. The density matrix formalism described in the following section will give us the tools to describe open systems. There is an alternative way to formulate Postulate 2, which describes the evolution of a system in continuous time.

\begin{postulate}{2'}
The time evolution of the state of a closed quantum system is
described by the Schrödinger equation,
\begin{equation}
    i \ \hbar \frac{d \ket{\psi}}{dt} = H \ket{\psi},
    \label{eq:postulate2p}
\end{equation}
\end{postulate}
where $\ \hbar$ is the reduced \emph{Planck constant} and $H$ is an Hermitian operator known as \emph{Hamiltonian} giving the energy of the physical system. Postulate 2 and Postulate 2' are equivalent because the unitary $U$ can always be written as
\begin{equation}
    U = e^{-i(t'-t)H/\hbar}
\end{equation}
due to the Hermitian character of the $H$ operator. 

The next postulate allows us to describe the interaction with a certain closed system, thereby enabling us to extract information from it.

\begin{postulate}{3}
Quantum measurements are characterized by a collection $\{M_m\}$ of measurement operators which satisfy
\begin{equation}
    \sum_m M_m^\dag M_m = \mathbb{I}.
    \label{completenessM}
\end{equation}
 These operators act on the state space of the state being measured. The index $m$ indicates the possible measurement outcomes that may occur in the experiment. The probability of result indexed by $m$ occurring when measuring state $\ket{\psi}$ is
 \begin{equation}
     p(m|\psi) = \bra{\psi}M_m^\dag M_m \ket{\psi},
 \end{equation}%
and the state after the measurement is 
\begin{equation}
    \frac{M_m \ket{\psi}}{\sqrt{p(m|\psi)}}.
\end{equation}
\end{postulate}
Equation \ref{completenessM} implies that the probabilities add up to one, thus forming a valid probability distribution
\begin{equation}
    \sum_m p(m|\psi) = \bra{\psi} \Big(\sum_m M_m^\dag M_m\Big) \ket{\psi}  = \braket{\psi} = 1 .
\end{equation}
Notice the fundamental difference between the time evolution and measurements of a quantum system. The temporal evolution is deterministic and reversible since every unitary operator is invertible. On the other hand, measurements are irreversible (the measurement operators are not unitary since the completeness relation $\sum_m M_m^\dag M_m = \mathbb{I}$ is incompatible with the unitary condition $M_m^\dag M_m = \mathbb{I} \ \forall m$). 

A special class of measurement operators are called \emph{projective measurements}. A projective measurement $\{P_m\}$ is described by an observable (an Hermitian operator) $A$ whose spectral decomposition is
\begin{equation}
    A = \sum_m a_m P_m, 
\end{equation}
where $a_m \in \mathbb{R}$ are the eigenvalues of $A$ and $P_m \geq 0$ are the projectors to the eigenspace of $a_m$. The only possible outcomes of the measurement are the eigenvalues $a_m$. In this case, the probabilities after the measurement are given by 
\begin{equation}
    p(m|\psi) = \bra{\psi} P_m \ket{\psi},
\end{equation}
and the state after the measurement is
\begin{equation}
    \frac{P_m \ket{\psi}}{\sqrt{ p(m|\psi) }}.
\end{equation}
Notice that a projective measurement $P_m$ is a subclass of a general measurement operator $M_m$. Since $P_m$ are projectors, they follow that $P_m = P_m^\dag$, $P_mP_l = \delta_{ml} P_m$ and $\sum_m P_m = \mathbb{I}$. Each $P_m$ can be interpreted as an elemental experiment which has a binary answer (YES or NO). A nice property of projective measurements is that the expected value of an operator can be easily calculated as
\begin{equation}
    \expval{A} \coloneqq \mathbb{E}(A|\psi) = \sum_m a_m p(m) = \sum_m a_m \bra{\psi} P_m \ket{\psi} = \bra{\psi} \Big(\sum_m a_m P_m\Big) \ket{\psi} = \bra{\psi} A \ket{\psi}. 
\end{equation}
The simplest example of projective measurement is the measurement of a qubit on the computational basis. The observable in this case would be the Pauli matrix $Z = \ketbra{0} - \ketbra{1}$. The projectors are then 
\begin{equation*}
    P_{+1} = \ketbra{0}, \quad P_{-1} = \ketbra{1}.
\end{equation*}
If the general state $\ket{\psi} = a \ket{0} + b\ket{1}$ is measured, then the probability of having the result $+1$ is either
\begin{equation*}
    p(+1|\psi)= \bra{\psi} P_{+1} \ket{\psi} = \bra{\psi}\ketbra{0}\ket{\psi} = |a|^2,
\end{equation*}
and similarly the probability of getting the output $-1$ is $p(-1|\psi) = |b|^2$. The state after the measurement in each case is 
\begin{equation*}
    \frac{\ketbra{0} \ket{\psi}}{|a|} = \frac{a}{|a|}\ket{0} = \ket{0}, \quad  \frac{\ketbra{1} \ket{\psi}}{|b|} = \ket{1},
\end{equation*}
where we have used that the global phase of the state can be ignored because of Postulate 1.

Another interesting class of measurement operators are called \gls{POVM} (Positive operator-valued measurement). In the cases where we are only interested in the result of the measurement, and not the state after the measurement (because we only want to measure it once, for instance) it is sufficient to use the POVM formalism. A POVM is characterized by a set of operators $\{E_m\}$ such that
\begin{enumerate}
    \item they are positive $\bra{\psi} E_m \ket{\psi} \geq 0 \quad \forall \ket{\psi}$,
    \item they fulfill the completeness relationship $\sum_m E_m = \mathbb{I}$,
    \item the probability of obtaining result indexed by $m$ given a state $\ket{\psi}$ is $p(m|\psi) = \bra{\psi}E_m\ket{\psi}$.
\end{enumerate}
A key difference between a projective measurement and a POVM is the repeatability property. Projective measurements are repeatable since after performing the measurement and obtaining result $m$, repeating the measurement will lead to result $m$ again and will not change the final state. However, there are many experiments which do not fulfill this property. For instance, measuring the position of the photon in a screen will likely destroy the photon, making it impossible to repeat the measurement. For this reason, general measurements need to be used when describing this kind of phenomenon.

The last postulate shows how to describe a system with two or more states.

\begin{postulate}{4}
The state space of a composite physical system is the tensor product of the state spaces of the component physical systems. Numbering the systems from 1 to n, and denoting the state in the system $i$ as $\ket{\psi_i}$, the joint state is 
\begin{equation}
    \ket{\Psi} = \ket{\psi_1} \otimes \ket{\psi_2} \otimes \cdots \otimes \ket{\psi_n}.
    \label{post4}
\end{equation}
\end{postulate}
Note that this definition is consistent with the superposition principle. If a bipartite system can be in state $\ket{\psi_1}\ket{\psi_2}$ and in state $\ket{\psi_1'}\ket{\psi_2'}$, then, because of superposition, in principle it should be allowed to be in state $a\ket{\psi_1}\ket{\psi_2} + b\ket{\psi_1}\ket{\psi_2}$. This property only makes sense in the tensor product space. Not all states, however, can be written as a tensor product of states (as in Eq. \ref{post4}).  Consider, for example, the state $\frac{1}{\sqrt{2}} (\ket{01} + \ket{10})$ (where the notation $\ket{01}$ refers to $\ket{0} \otimes \ket{1}$). It is easy to prove that this state can not be written as a product state $\ket{\psi}\ket{\phi}$. 

We say that any state which can not be written as the tensor product of states is an \emph{entangled} state. Interestingly, entangled states play a fundamental role in quantum computing and quantum information, as they are the key to many algorithms and protocols. Entanglement allows multiple qubits to be connected so that the state of one qubit depends on the state of the others. This allows quantum computers to perform certain operations that are not possible on classical computers, allowing for much more efficient computation. 

In quantum computing, entanglement is used to perform quantum algorithms, such as Shor's algorithm for factorization \citep{Shor}, and Grover's algorithm for search problems \citep{Grover}, where the use of entangled states allows for significant speed-ups compared to classical algorithms. Entanglement also plays a critical role in QML, where the use of entangled states allows the processing of large amounts of data with fewer quantum computational resources.

\subsection{The density matrix}
It is often the case that only partial knowledge of the state of a physical system is available. This can happen for many reasons, such as the imperfections of experimental devices or the coupling of the system of interest with its environment. In these situations, the system can be described through the \emph{density matrix}. 

Suppose that a quantum system is in state $\ket{\psi_i}$ with probability $p_i$, for $i=1, \cdots, N$. The set $\{p_i, \ket{\psi_i}\}$ is called an \emph{ensemble of pure states}. The density matrix is defined as
\begin{equation}
    \rho = \sum_i p_i \ketbra{\psi_i},
\end{equation}
and we say that $\rho$ is a \emph{mixed state}. On the other hand, when the quantum state $\ket{\psi}$ is known exactly (i.e. with $p=1$) we say that $\ket{\psi}$ is a \emph{pure state}. The density matrix of a pure state is simply $\rho = \ketbra{\psi}$. 

Now an interesting question arises. How do we differentiate between pure and mixed states? A density matrix $\rho$ represents a pure state if and only if $\tr \rho^2 = 1$. Otherwise, $\tr \rho^2 < 1$. For this reason, the quantity $\tr \rho^2$ is called the \emph{purity} of a density matrix. It can be easily shown that any matrix $\rho$ is a density matrix if and only if $\rho$ is positive with trace equal to one. 

Now, the postulates of quantum mechanics that we defined in the previous section can be reformulated in terms of the density matrix.
\begin{postulate}{1}
Associated with any closed physical system is a Hilbert space $\mathcal{H}$ known as the state space of the system. The system is completely described by its density matrix, which is a
positive, trace-one operator acting on the state space of the system.
\end{postulate}
For one-qubit systems, a general density matrix can be written as a linear combination of Pauli operators 
\begin{equation}
    \rho = \frac{\mathbb{I} + r_x X + r_y Y + r_z Z}{2}, \quad ||(r_x, r_y, r_z)|| \leq 1,
\end{equation}
where $||(r_x, r_y, r_z)||=1$ only if $\rho$ is a pure state, recovering Eq. \ref{eq:pure_state_Pauli_decomposition}. 
\begin{postulate}{2}
The evolution of a closed quantum system is unitary. That is, if the quantum state of a closed system is $\rho$ at time $t$ and $\rho'$ at time $t'$, then
\begin{equation}
    \rho' = U \rho U^\dag,
\end{equation}
where $U$ is a unitary operator which depends only on $t' - t$.
\end{postulate}
\begin{postulate}{3}
Quantum measurements are characterized by a collection $\{M_m\}$ of measurement operators which satisfy
\begin{equation}
    \sum_m M_m^\dag M_m = \mathbb{I}.
\end{equation}
 These operators act on the state space of the state being measured. The index $m$ indicates the measurement outcomes that may occur in the experiment. The probability of result $m$ occurring when measuring state $\ket{\psi}$ is
 \begin{equation}
     p(m|\rho) = \tr (M_m^\dag M_m \rho).
 \end{equation}
And the state after the measurement is 
\begin{equation}
    \frac{M_m \rho M_m^\dag}{\sqrt{p(m|\rho)}}.
\end{equation}
\end{postulate}
\begin{postulate}{4}
The state space of a composite physical system is the tensor product of the state spaces of the component physical systems. Numbering the systems from 1 to n, and denoting the state in system $i$ as $\rho_i$, the joint state is 
\begin{equation}
    \rho = \rho_1 \otimes \rho_2 \otimes \cdots \otimes \rho_n.
\end{equation}
\end{postulate}
One of the most useful aspects of the density matrix formalism is the description of a subsystem of a composite quantum system. Consider a bipartite system composed of systems A and B. Suppose we do not have access to subsystem B (maybe because it is too far away). Then, we describe the state of system A using the \emph{reduced} density operator
\begin{equation}
    \rho^A \coloneqq \tr_B(\rho^{AB}),
    \label{partial_trace}
\end{equation}
where $\tr_B(\cdot)$ is the \emph{partial trace} over system B. The partial trace is a linear map defined as
\begin{equation}
    \tr_B(\ketbra{\psi_1}{\psi_2} \otimes \ketbra{\phi_1}{\phi_2} ) = \ketbra{\psi_1}{\psi_2} \tr(\ketbra{\phi_1}{\phi_2} ).
\end{equation}
The partial trace is chosen as the reduced density operator because it provides the correct outputs of the measurements made in the reduced subsystem. That is, given an operator $H \otimes \mathbb{I}$ acting only on system A, the definition in Eq. \ref{partial_trace} satisfies $\tr(H\rho^A) = \tr((H \otimes \mathbb{I})\rho^{AB})$. Let us consider two examples of composite states:

\begin{enumerate}
    \item Consider the state $\rho^{AB} = \rho^A \otimes \rho^B$, with $\rho^A = \ketbra{\psi}$. In this case, $\tr_B\rho^{AB} = \rho^A\tr \rho^B = \ketbra{\psi} $. In this situation, system B does not affect system A. Even ignoring the knowledge of system B, system A is already a pure state. There is no action that we can do to system B that can affect system A. And even though the original state was a mixed state, when tracing out system B we obtain a pure state in system A.
    
    \item Consider the opposite situation. Let the state of the system AB be
    \begin{equation*}
        \ket{\psi}_{AB} = \frac{1}{\sqrt{2}}(\ket{00} + \ket{11}).
    \end{equation*}
    The density matrix is 
    \begin{equation*}
        \rho = \frac{1}{2}(\ket{00} + \ket{11})(\bra{00} + \bra{11}) = \frac{1}{2} (\ketbra{00} + \ketbra{11}{00} + \ketbra{00}{11} + \ketbra{11}),
    \end{equation*}
    and the reduced state of system A is then
    \begin{equation*}
        \rho^A = \tr_B(\rho^{AB}) = \frac{1}{2}(\ketbra{00} + \ketbra{11}) = \frac{1}{2}\mathbb{I}.
    \end{equation*}
    The state of system A is therefore a \emph{maximally mixed state} (a random mixture of the orthonormal states $\{\ket{00}, \ket{11}\}$ with the same probability). Notice that the joint state $\ket{\psi}_{AB}$ is an entangled state. For a maximally entangled state, the correlations of the two subsystems are so strong that if we do not have access to the joint system, we do not know anything about the individual subsystems.
    
\end{enumerate}
